# Supplementary material for: A New Reference Chemical Composition for TMC-1
Source: arXiv:1610.00524 source file (2016-10-03)
Supplement: Supplementary file 1 [file appendix_figure_iso.tex]

\begin{figure*}
\includegraphics[width=16cm]{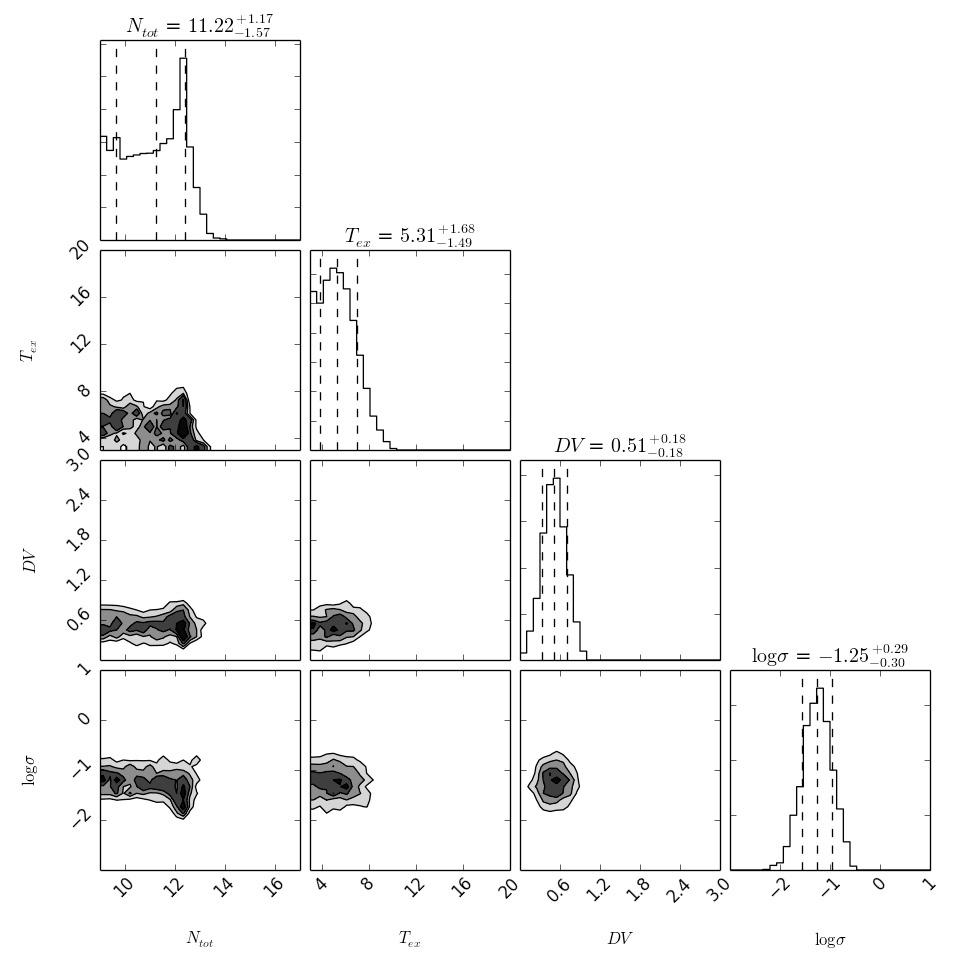}
\includegraphics[width=8cm]{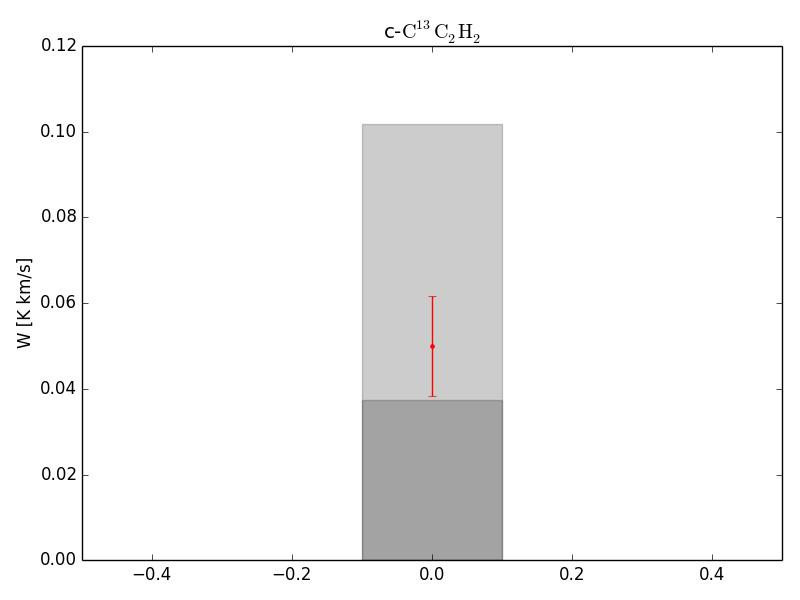}
\includegraphics[width=8cm]{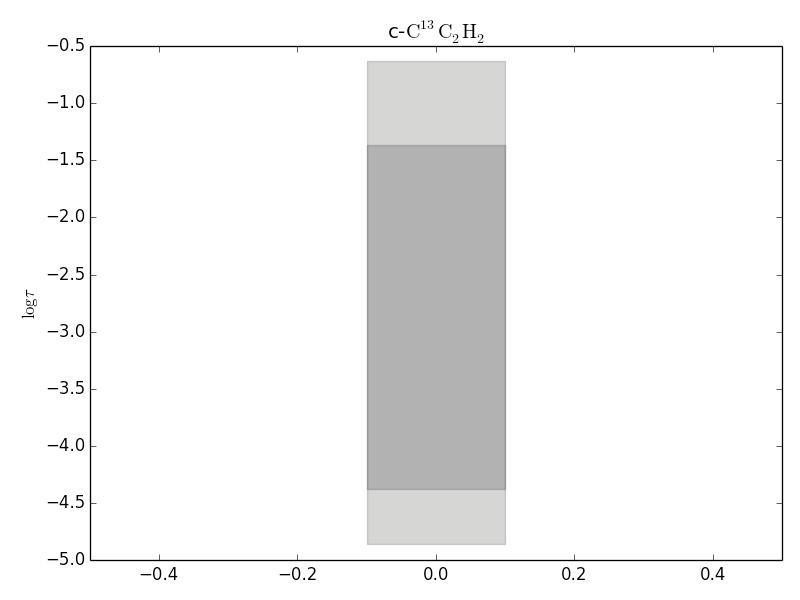}
\caption{\chem{^{13}CCH_2}}
\label{C13CCH2}
\end{figure*}
\clearpage
\begin{figure*}
\includegraphics[width=16cm]{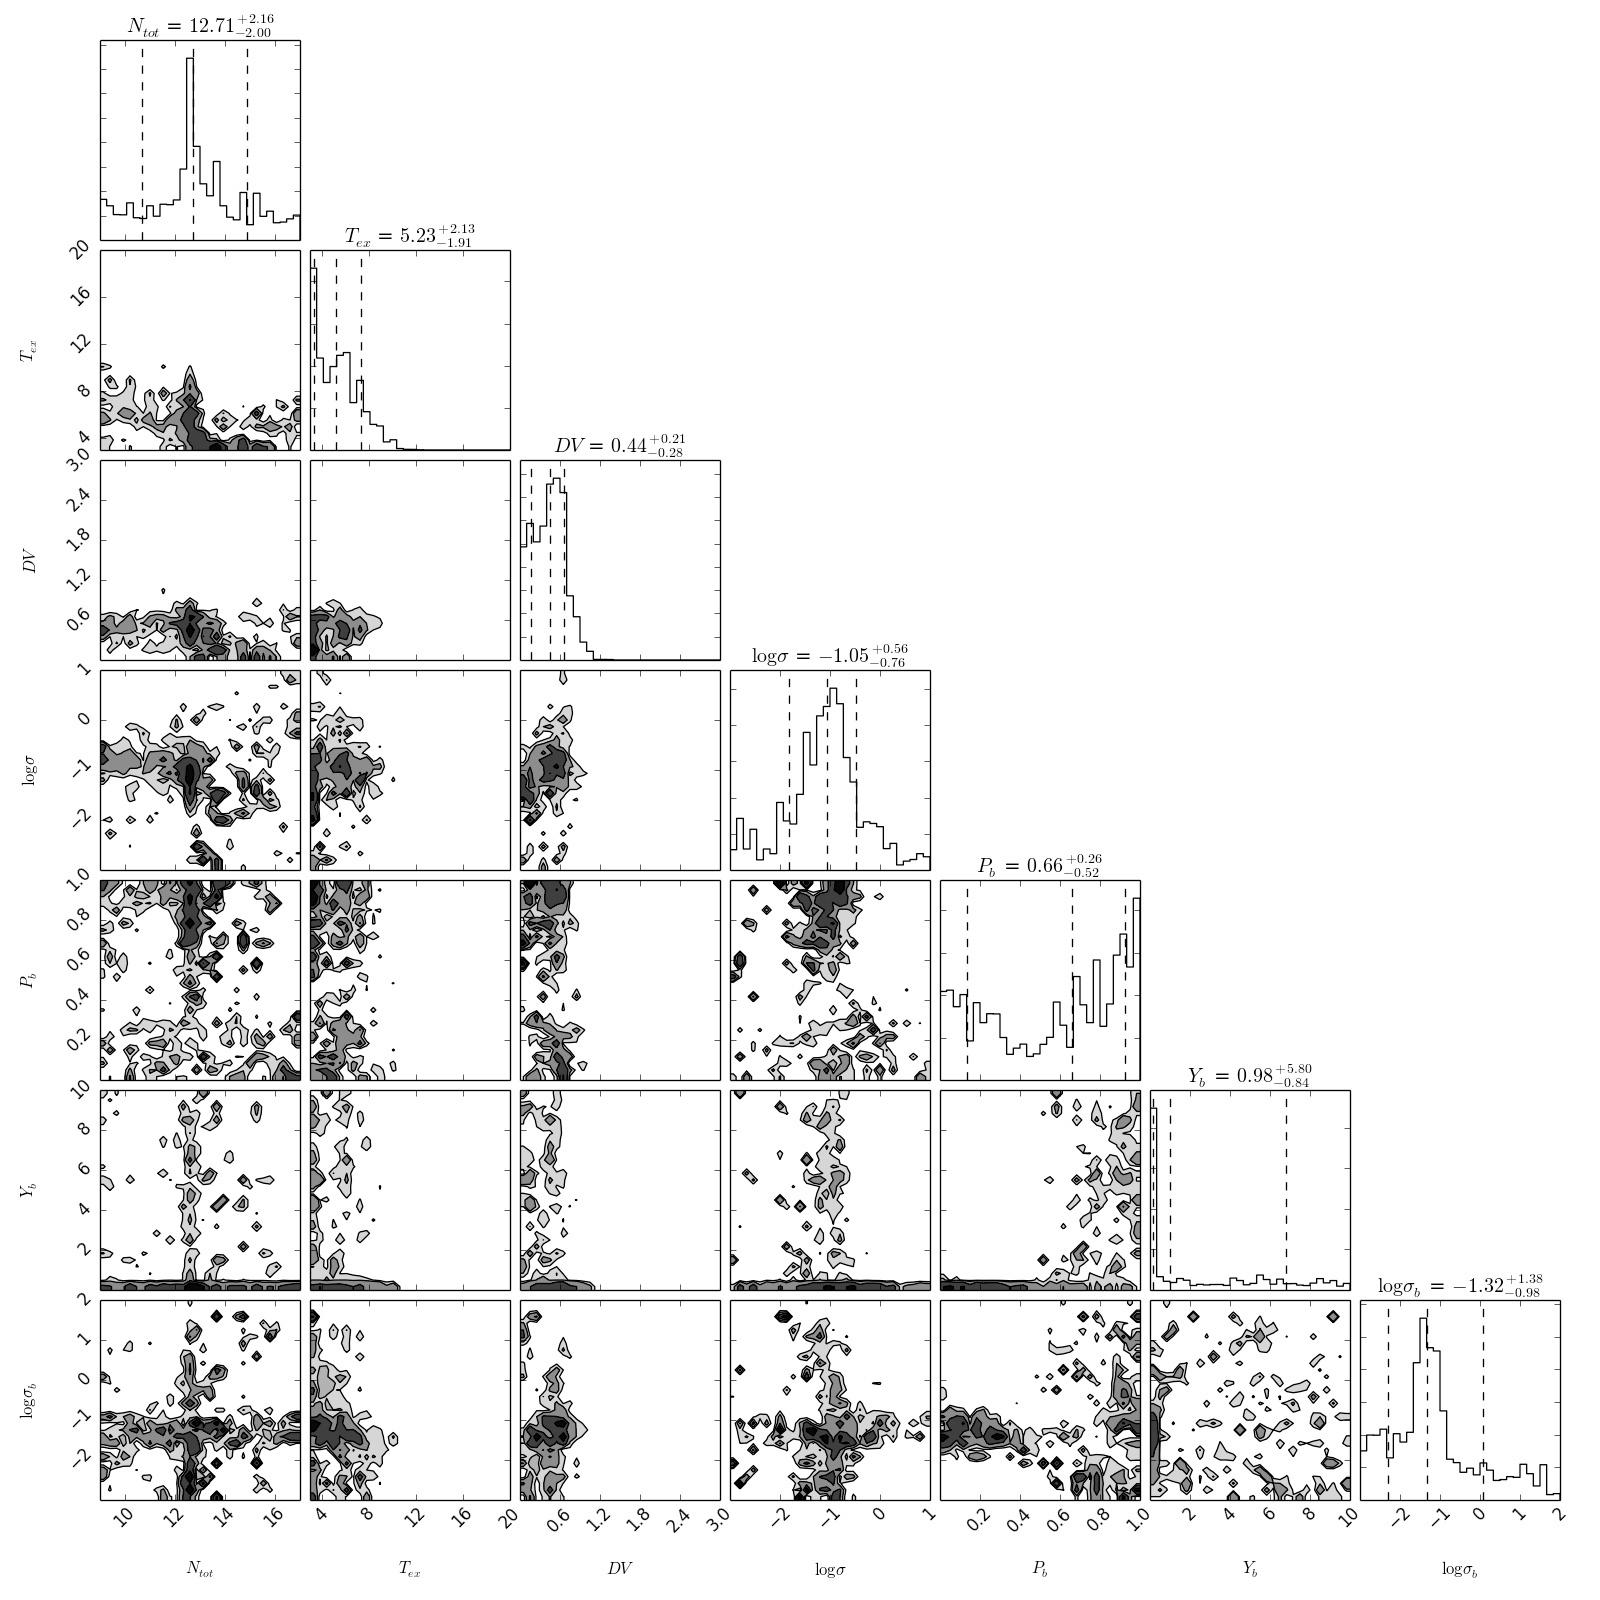}
\includegraphics[width=8cm]{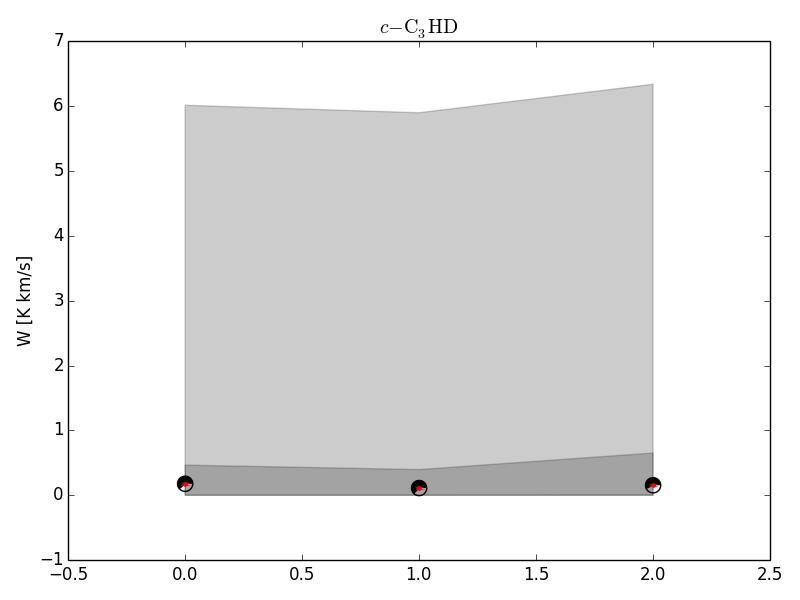}
\includegraphics[width=8cm]{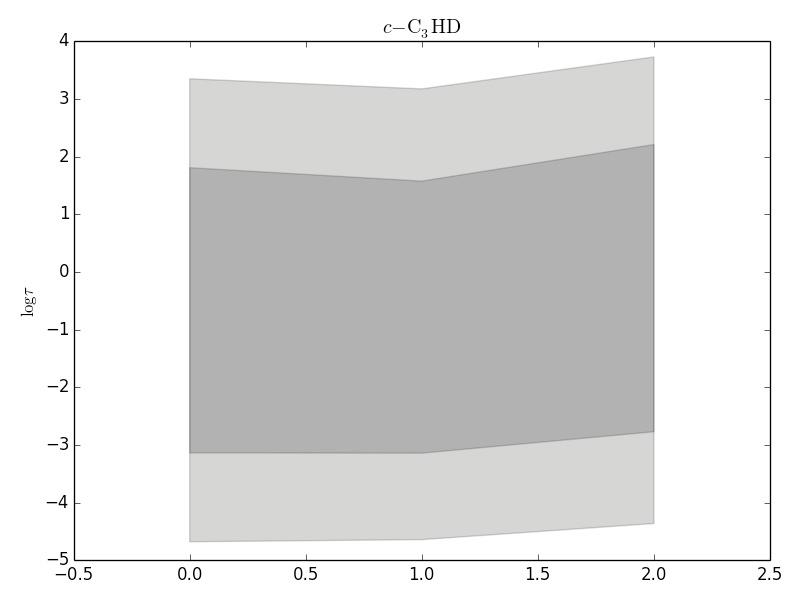}
\caption{\mbox{c-}\chem{C_3HD}}
\label{C3HD}
\end{figure*}
\clearpage
\begin{figure*}
\includegraphics[width=16cm]{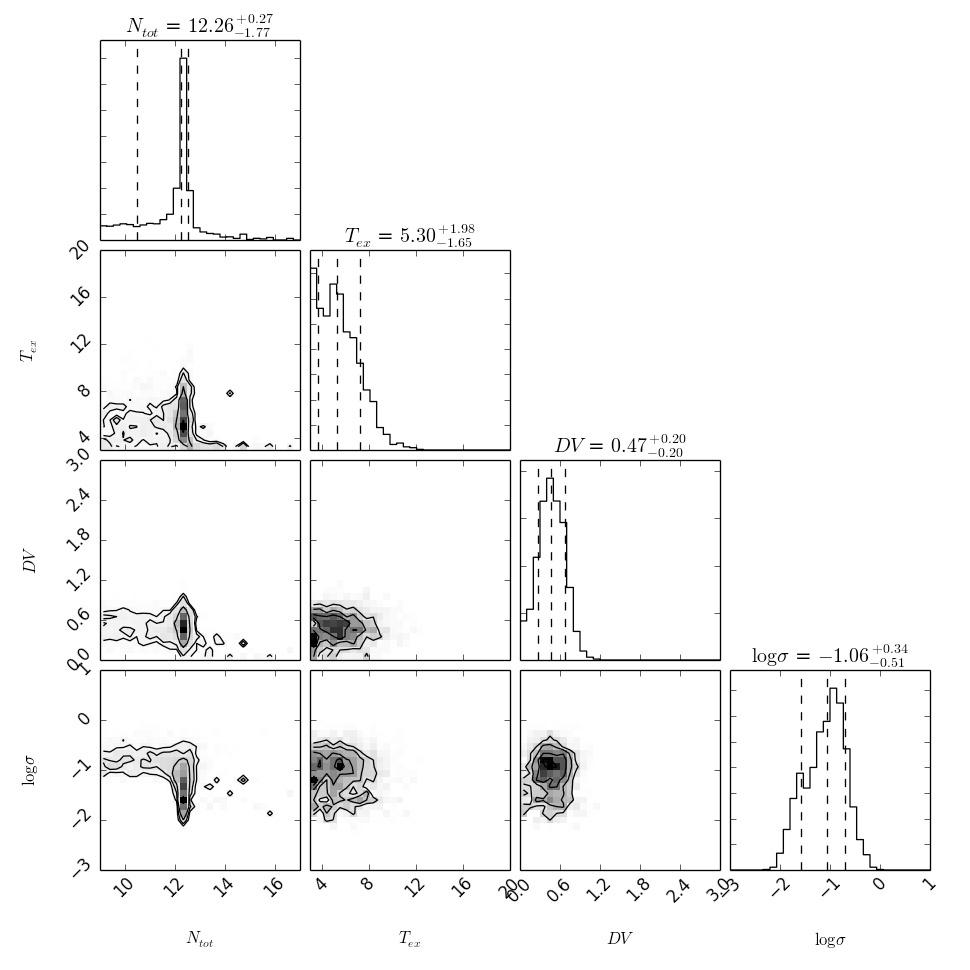}
\includegraphics[width=8cm]{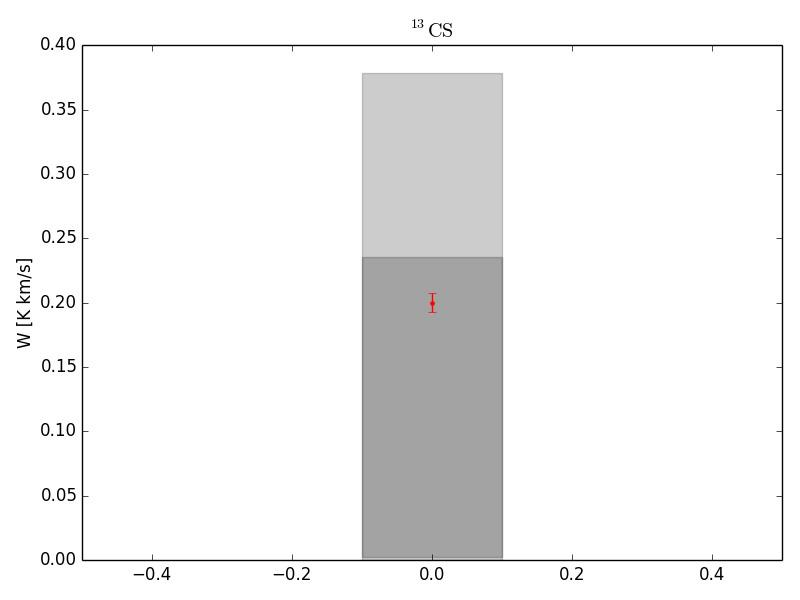}
\includegraphics[width=8cm]{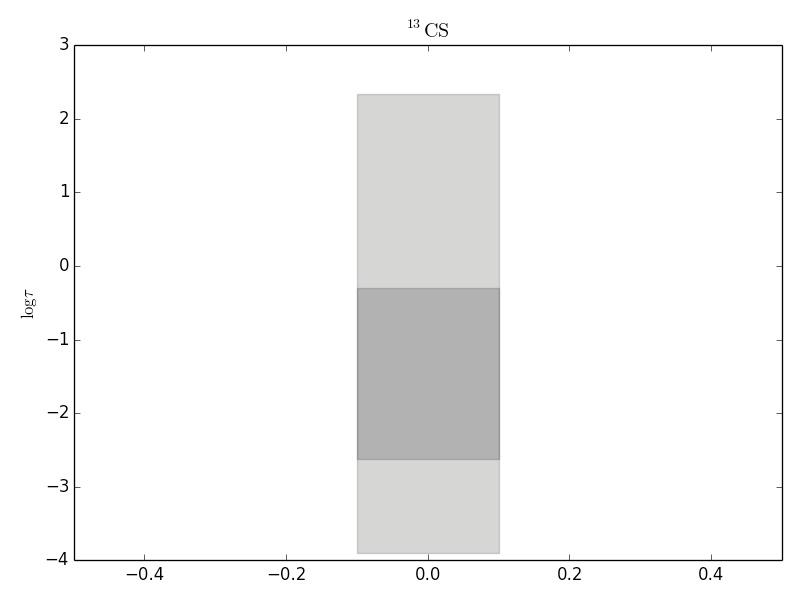}
\caption{\chem{^{13}CS}}
\label{thCS}
\end{figure*}
\clearpage
\begin{figure*}
\includegraphics[width=16cm]{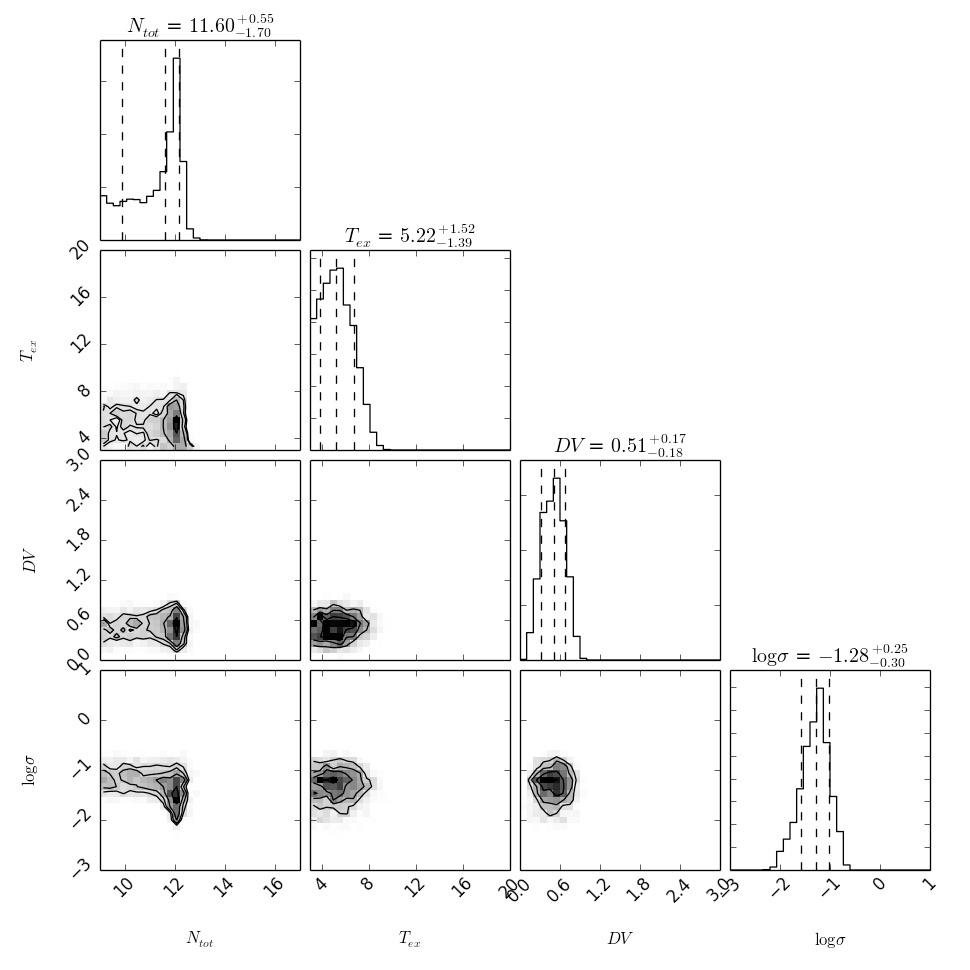}
\includegraphics[width=8cm]{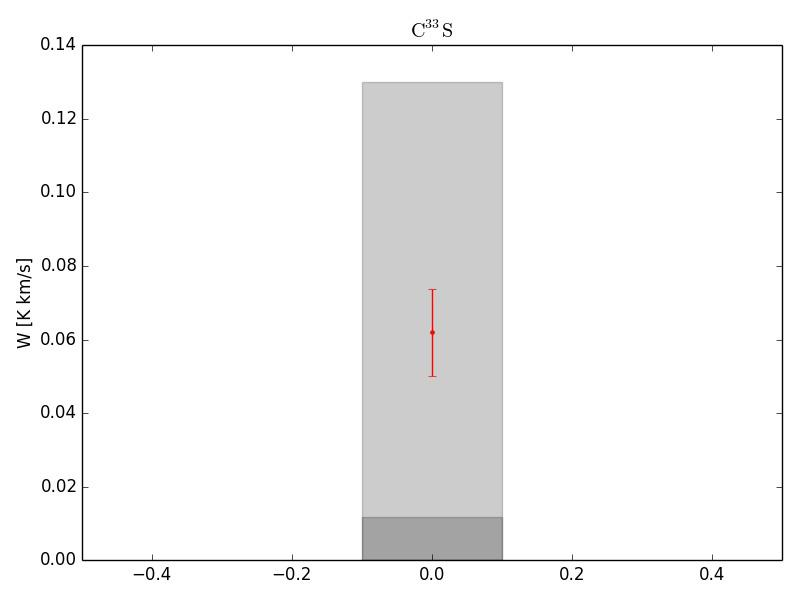}
\includegraphics[width=8cm]{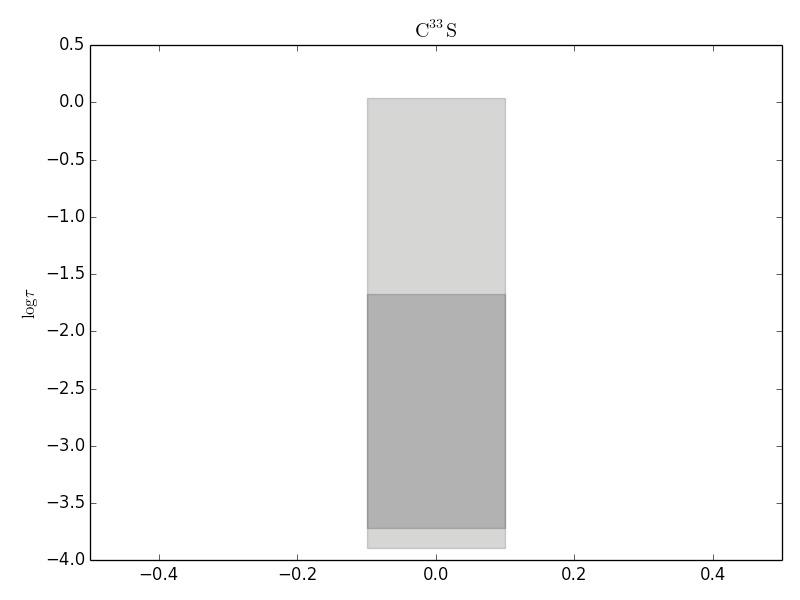}
\caption{\chem{C^{33}S}}
\label{C33S}
\end{figure*}
\clearpage
\begin{figure*}
\includegraphics[width=16cm]{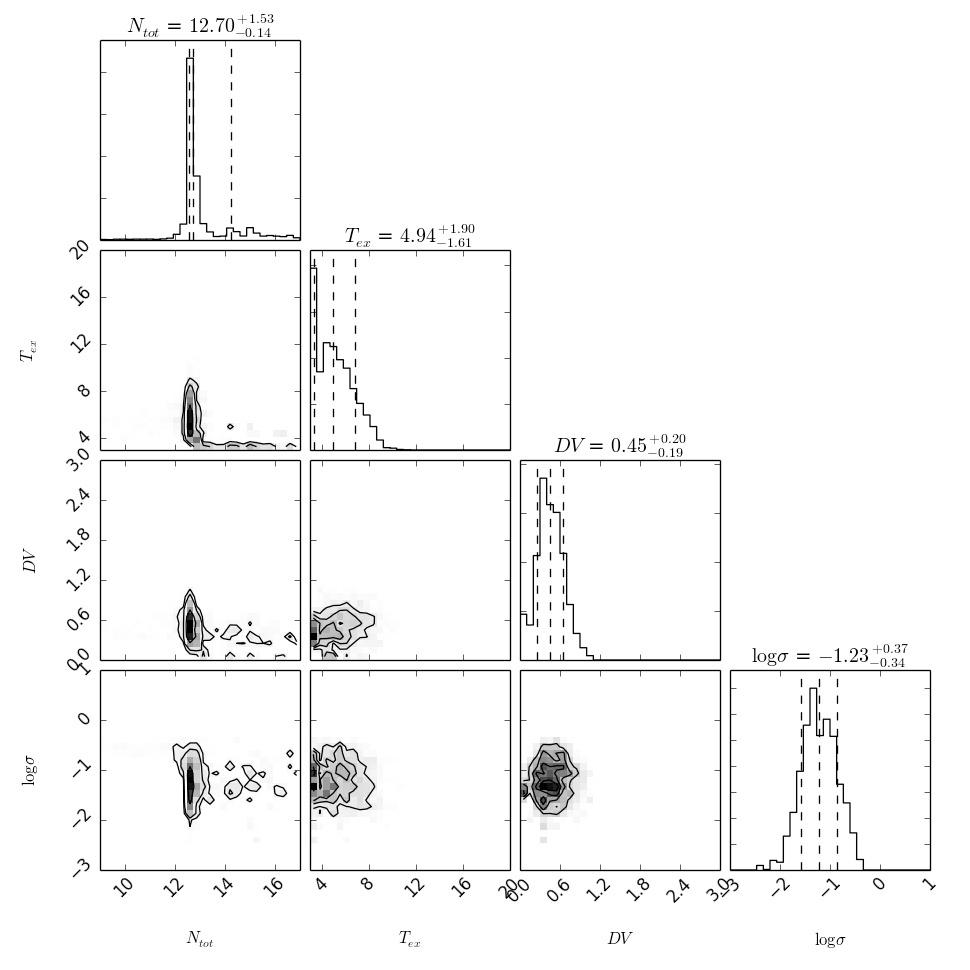}
\includegraphics[width=8cm]{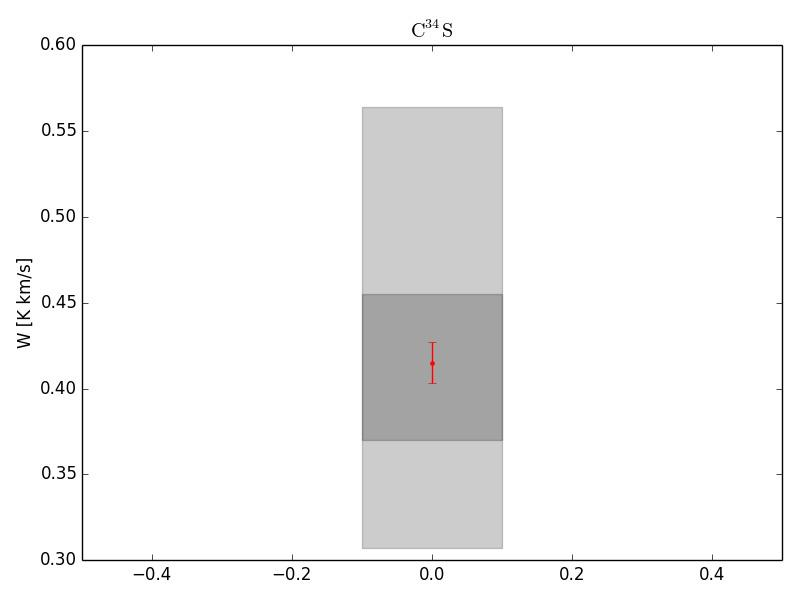}
\includegraphics[width=8cm]{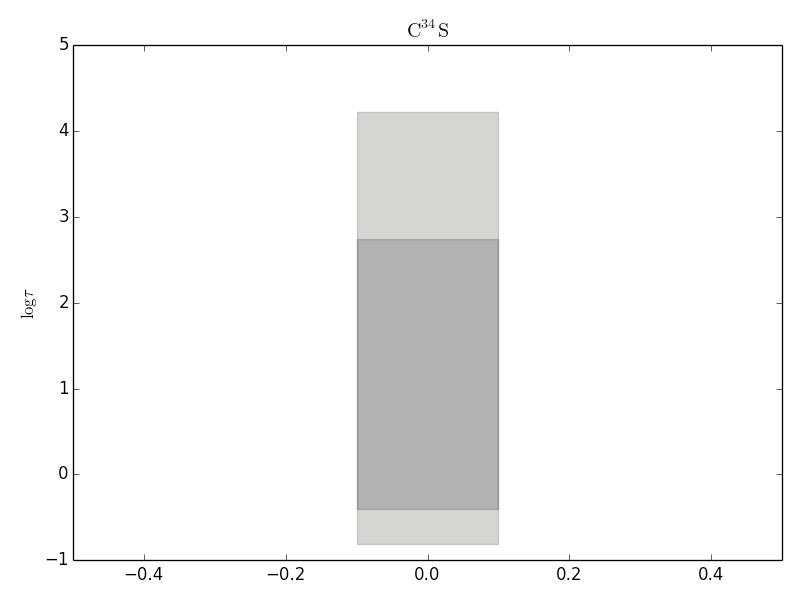}
\caption{\chem{C^{34}S}}
\label{C34S}
\end{figure*}
\clearpage
\begin{figure*}
\includegraphics[width=16cm]{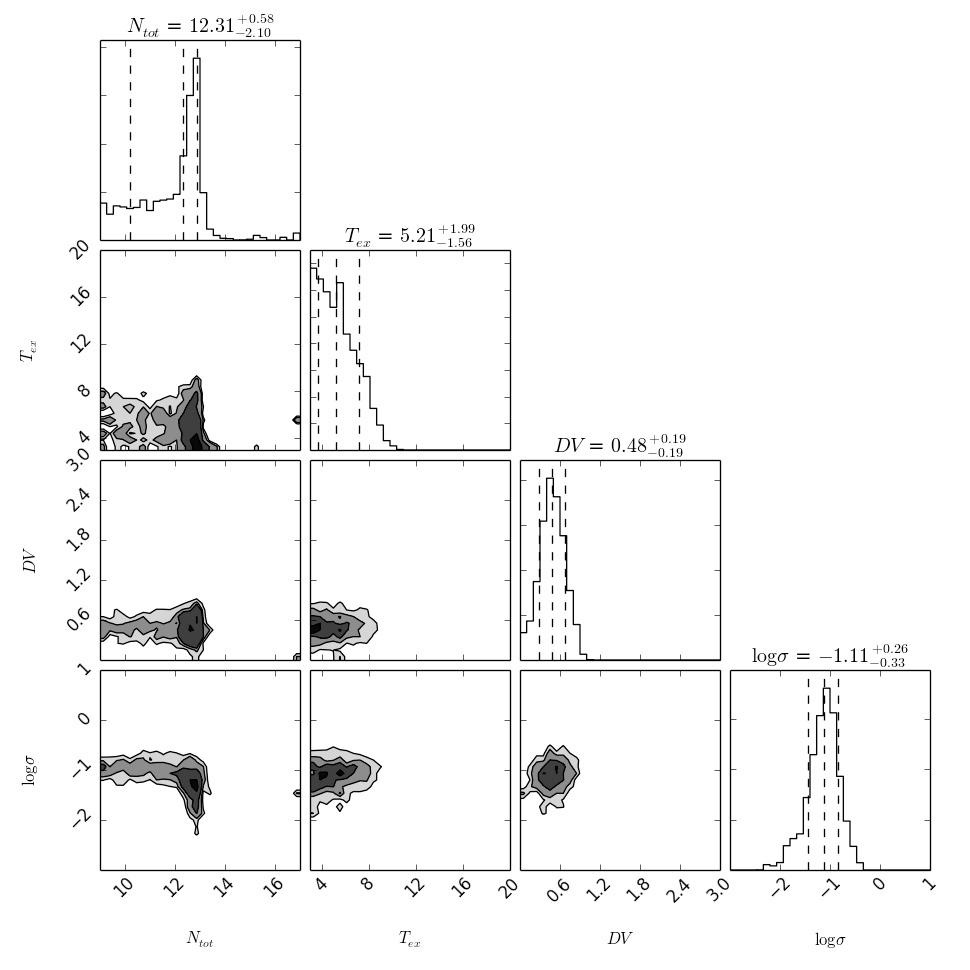}
\includegraphics[width=8cm]{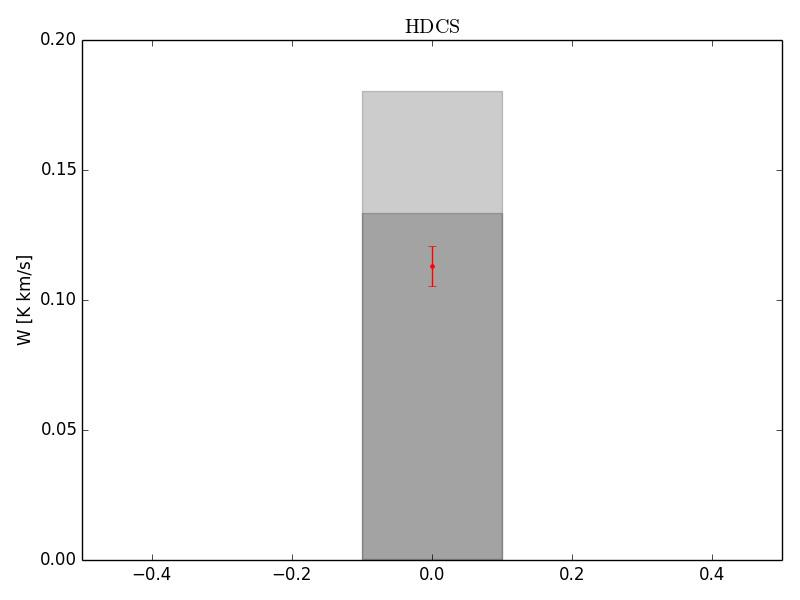}
\includegraphics[width=8cm]{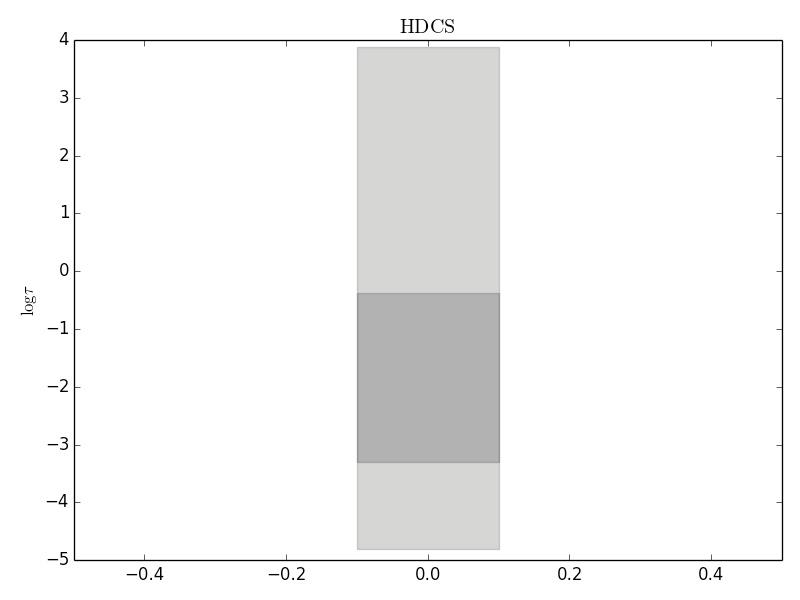}
\caption{\chem{HDCS}}
\label{HDCS}
\end{figure*}
\clearpage
\begin{figure*}
\includegraphics[width=16cm]{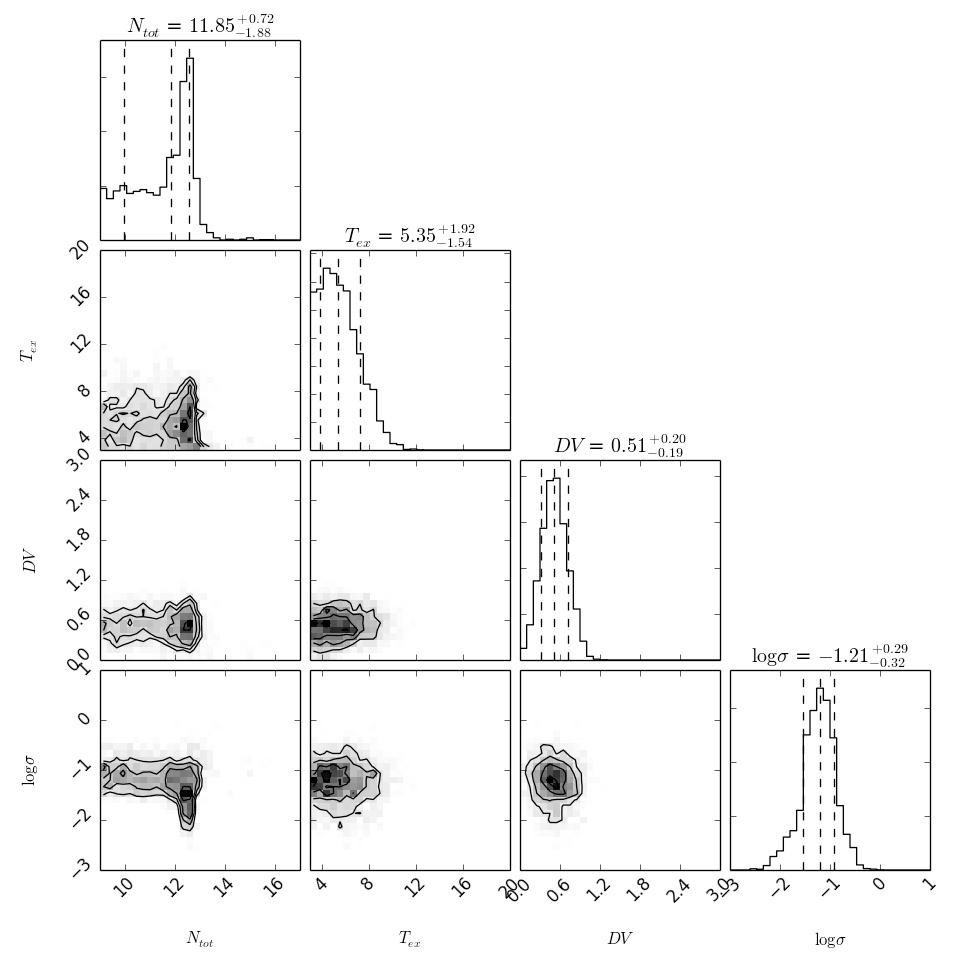}
\includegraphics[width=8cm]{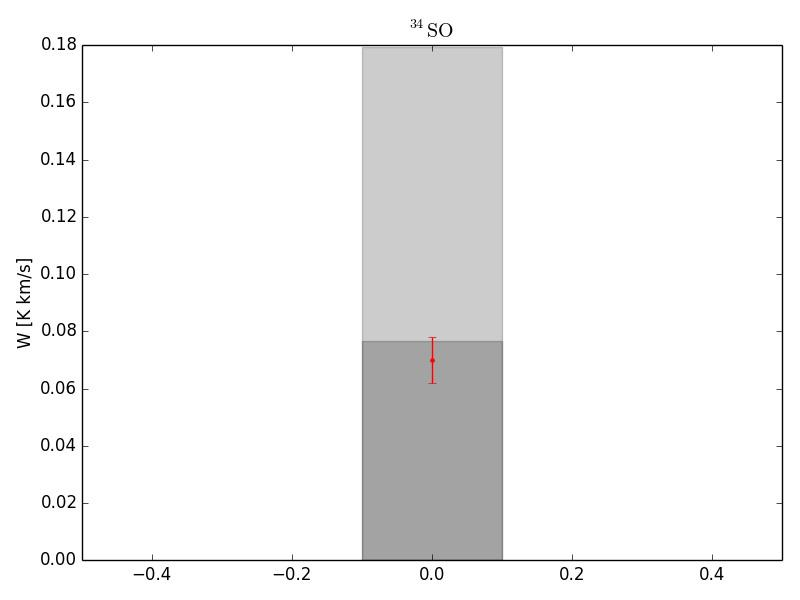}
\includegraphics[width=8cm]{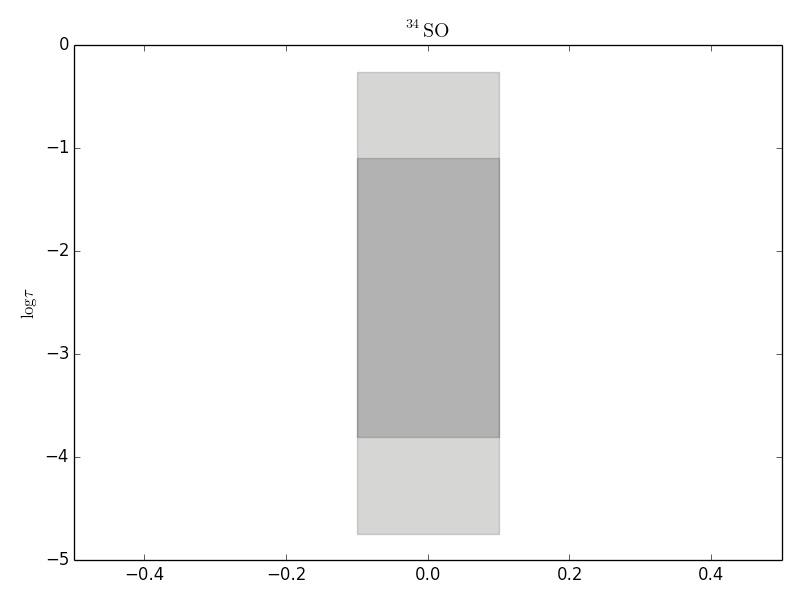}
\caption{\chem{^{34}SO}}
\label{34SO}
\end{figure*}
\clearpage
\begin{figure*}
\includegraphics[width=16cm]{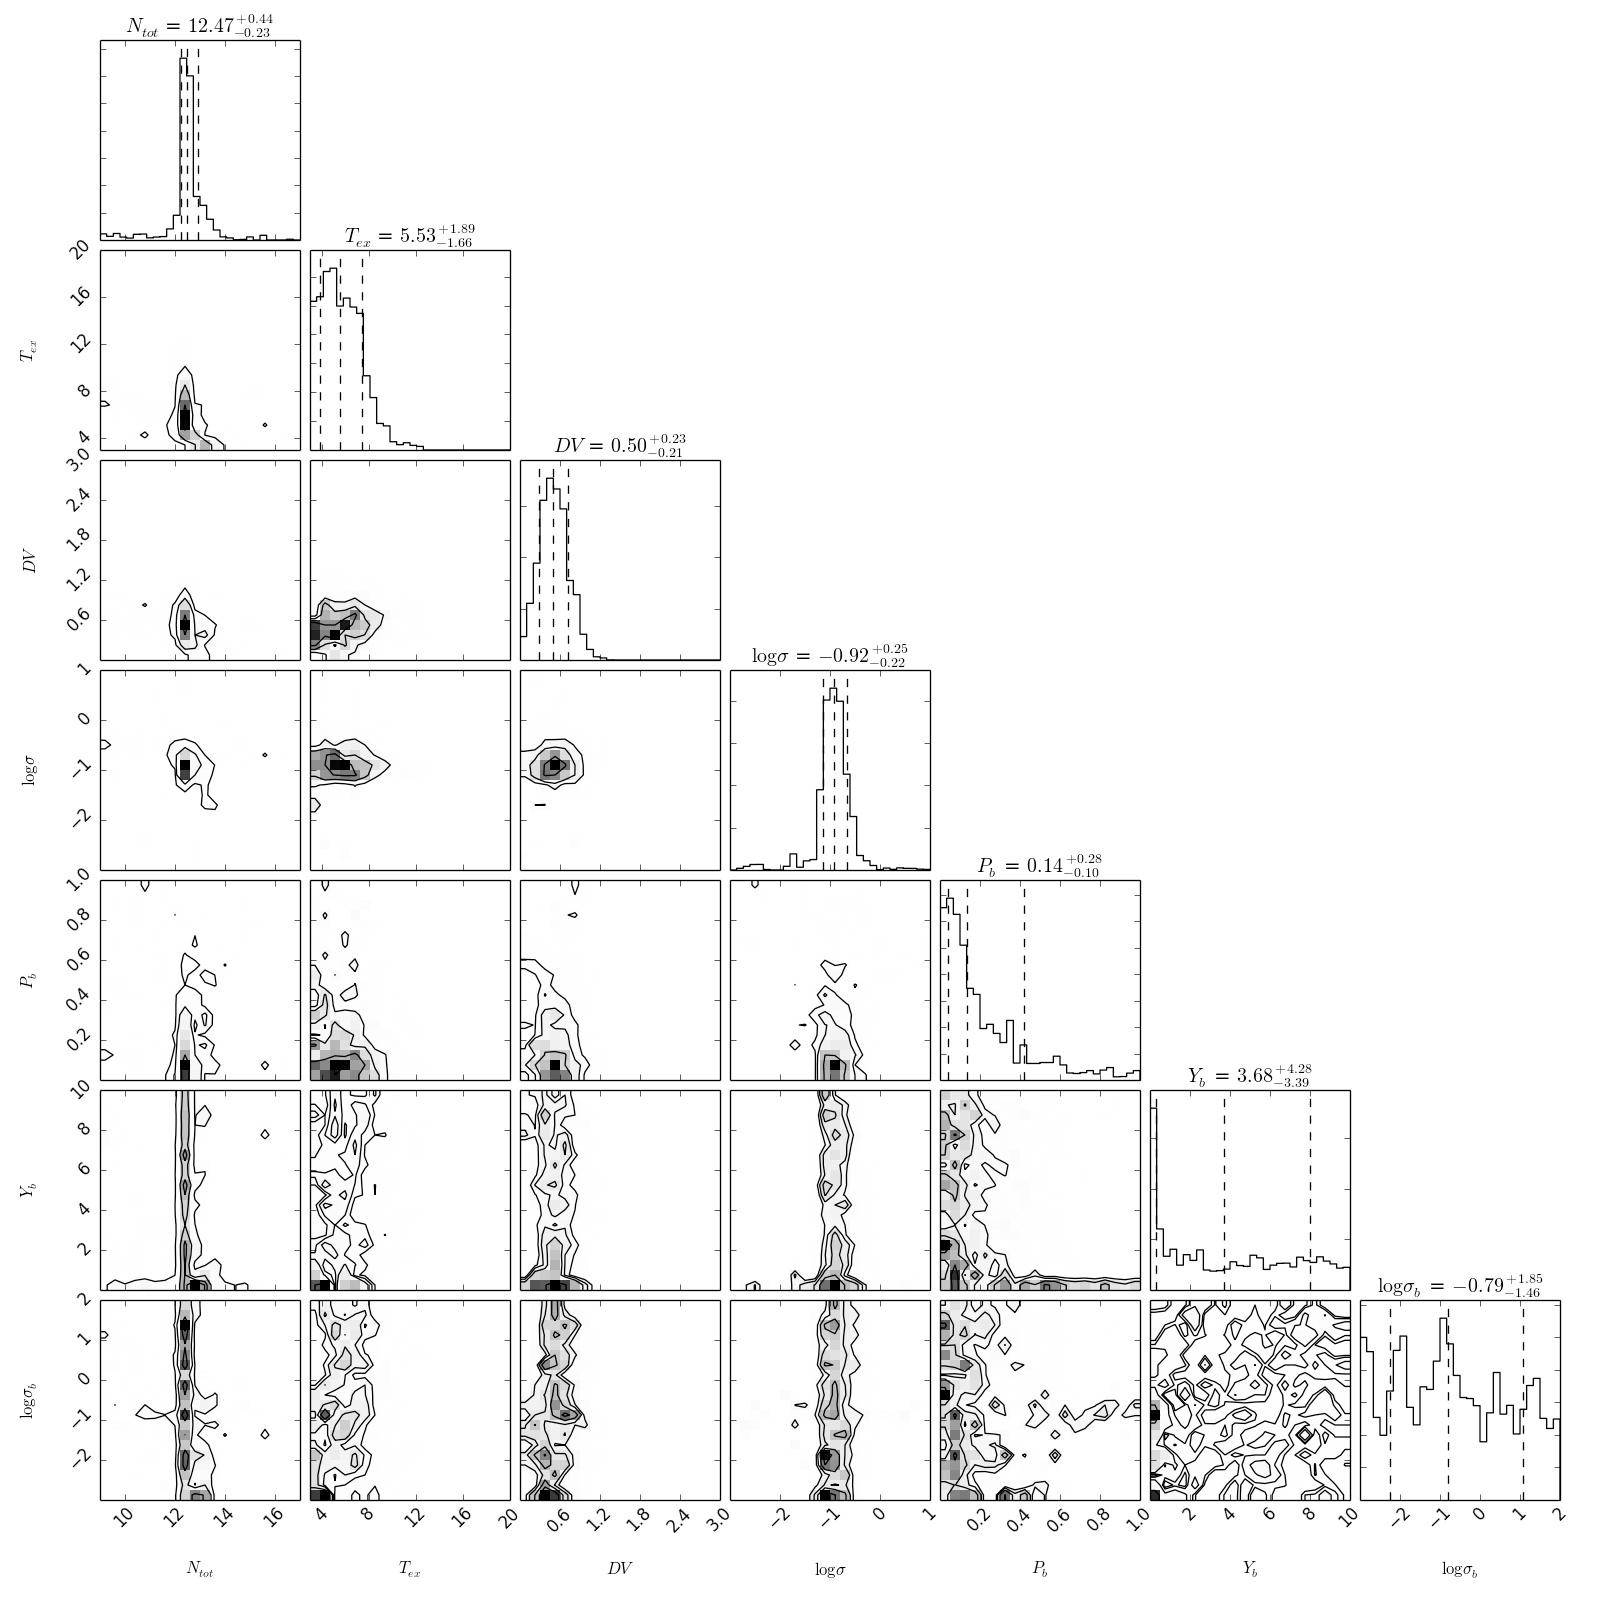}
\includegraphics[width=8cm]{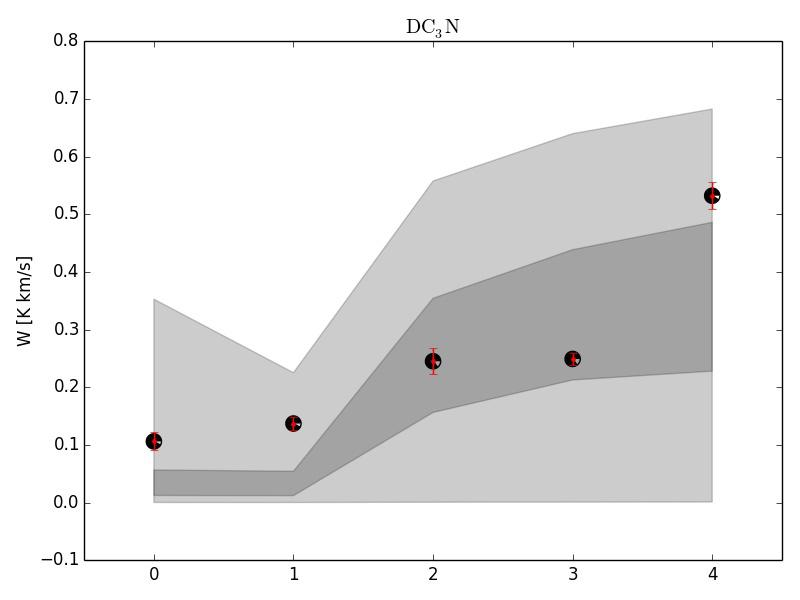}
\includegraphics[width=8cm]{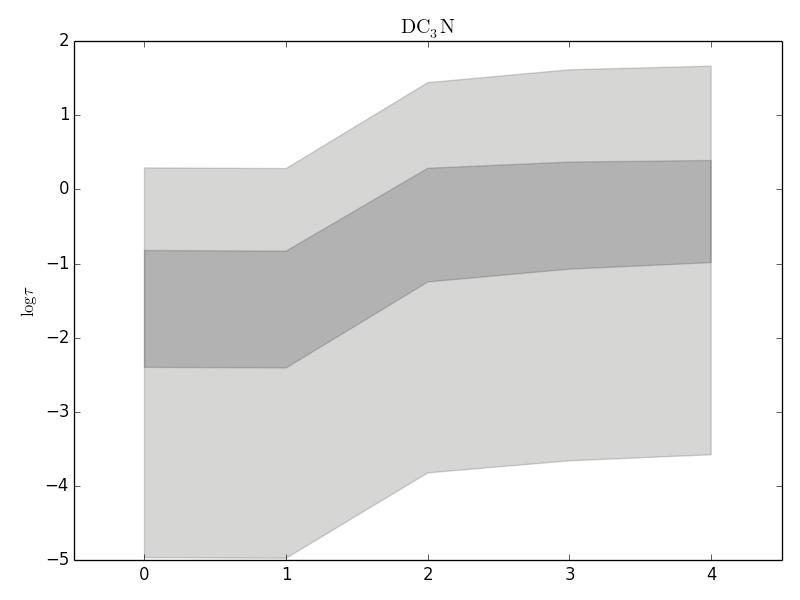}
\caption{\chem{DC_3N}}
\label{DC3N}
\end{figure*}
\clearpage
\begin{figure*}
\includegraphics[width=16cm]{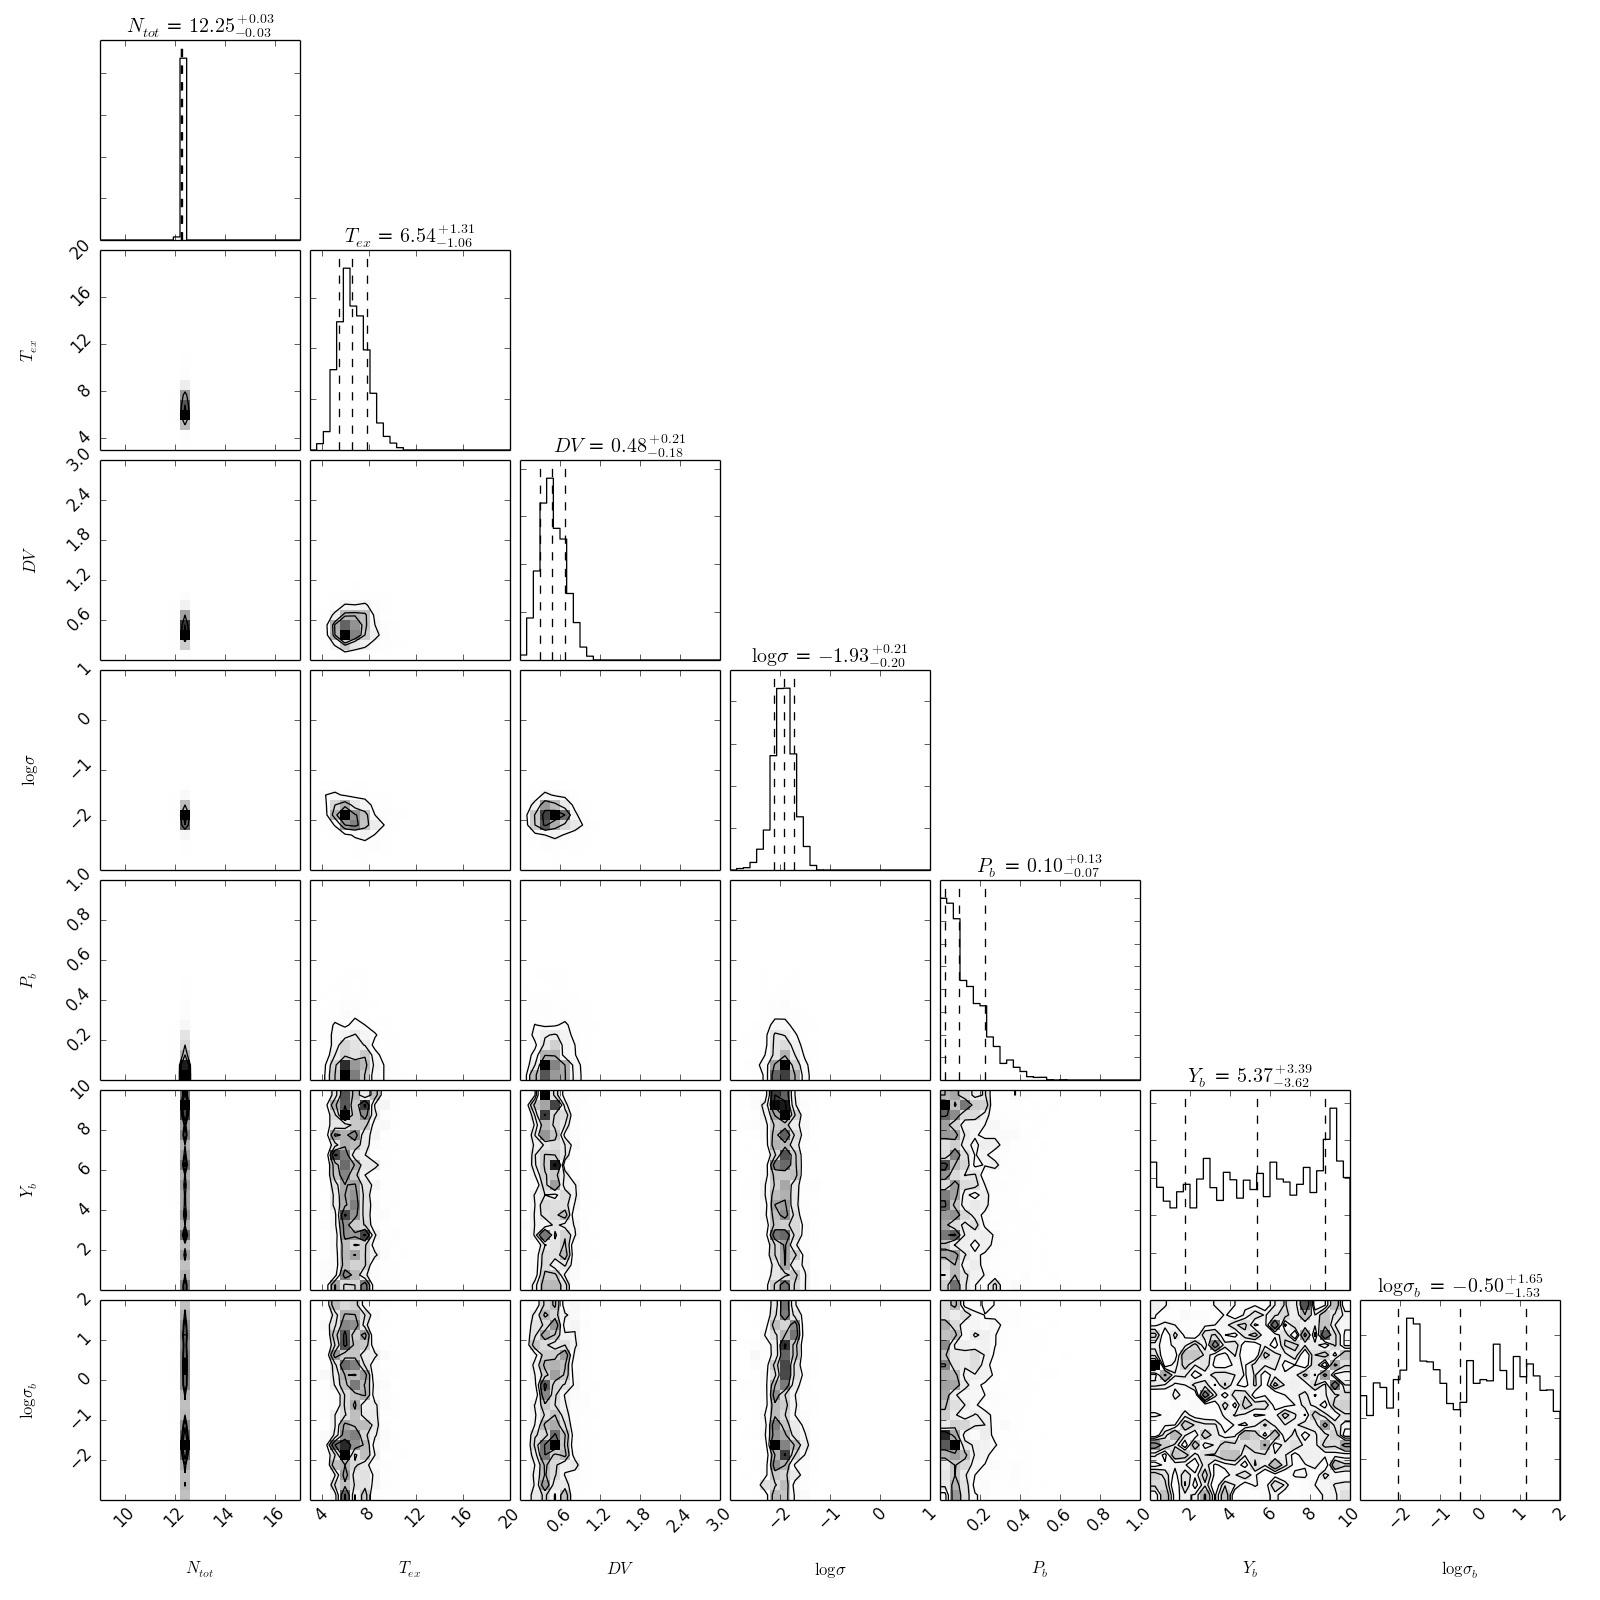}
\includegraphics[width=8cm]{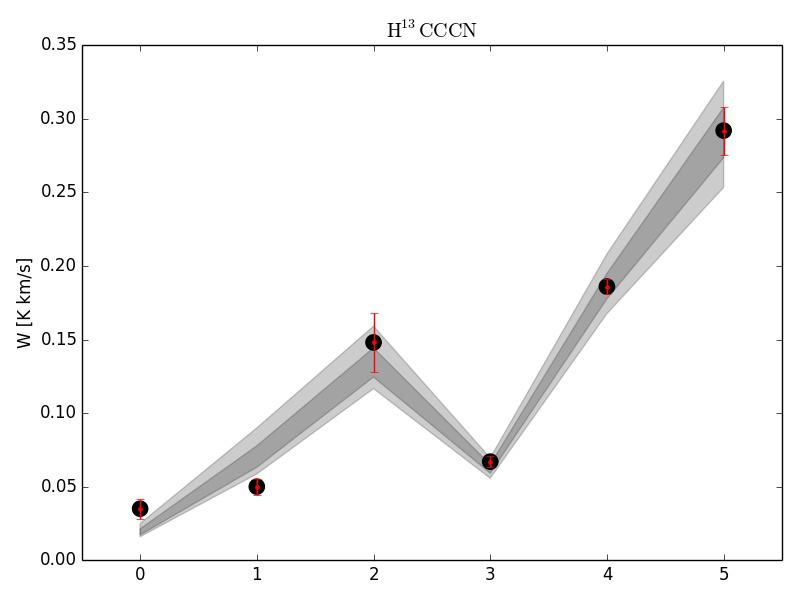}
\includegraphics[width=8cm]{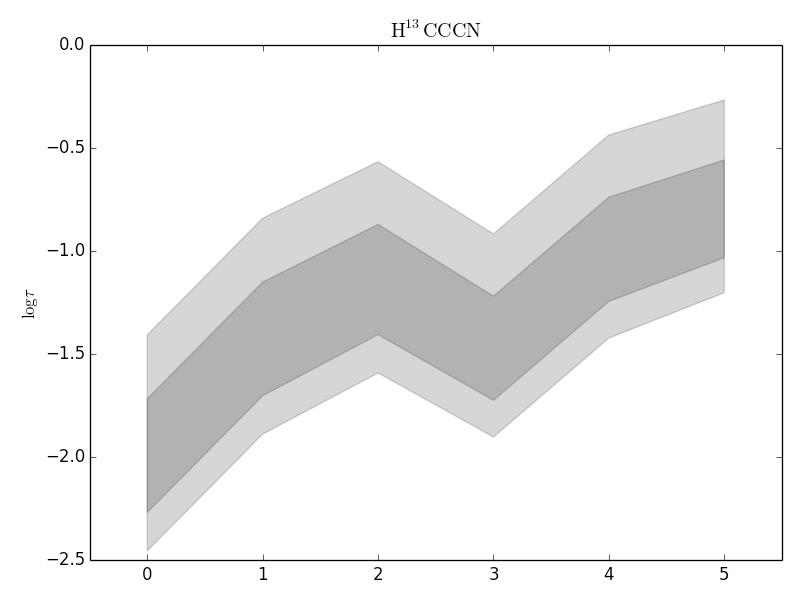}
\caption{\chem{H^{13}CC_2N}}
\label{H13CCCN}
\end{figure*}
\clearpage
\begin{figure*}
\includegraphics[width=16cm]{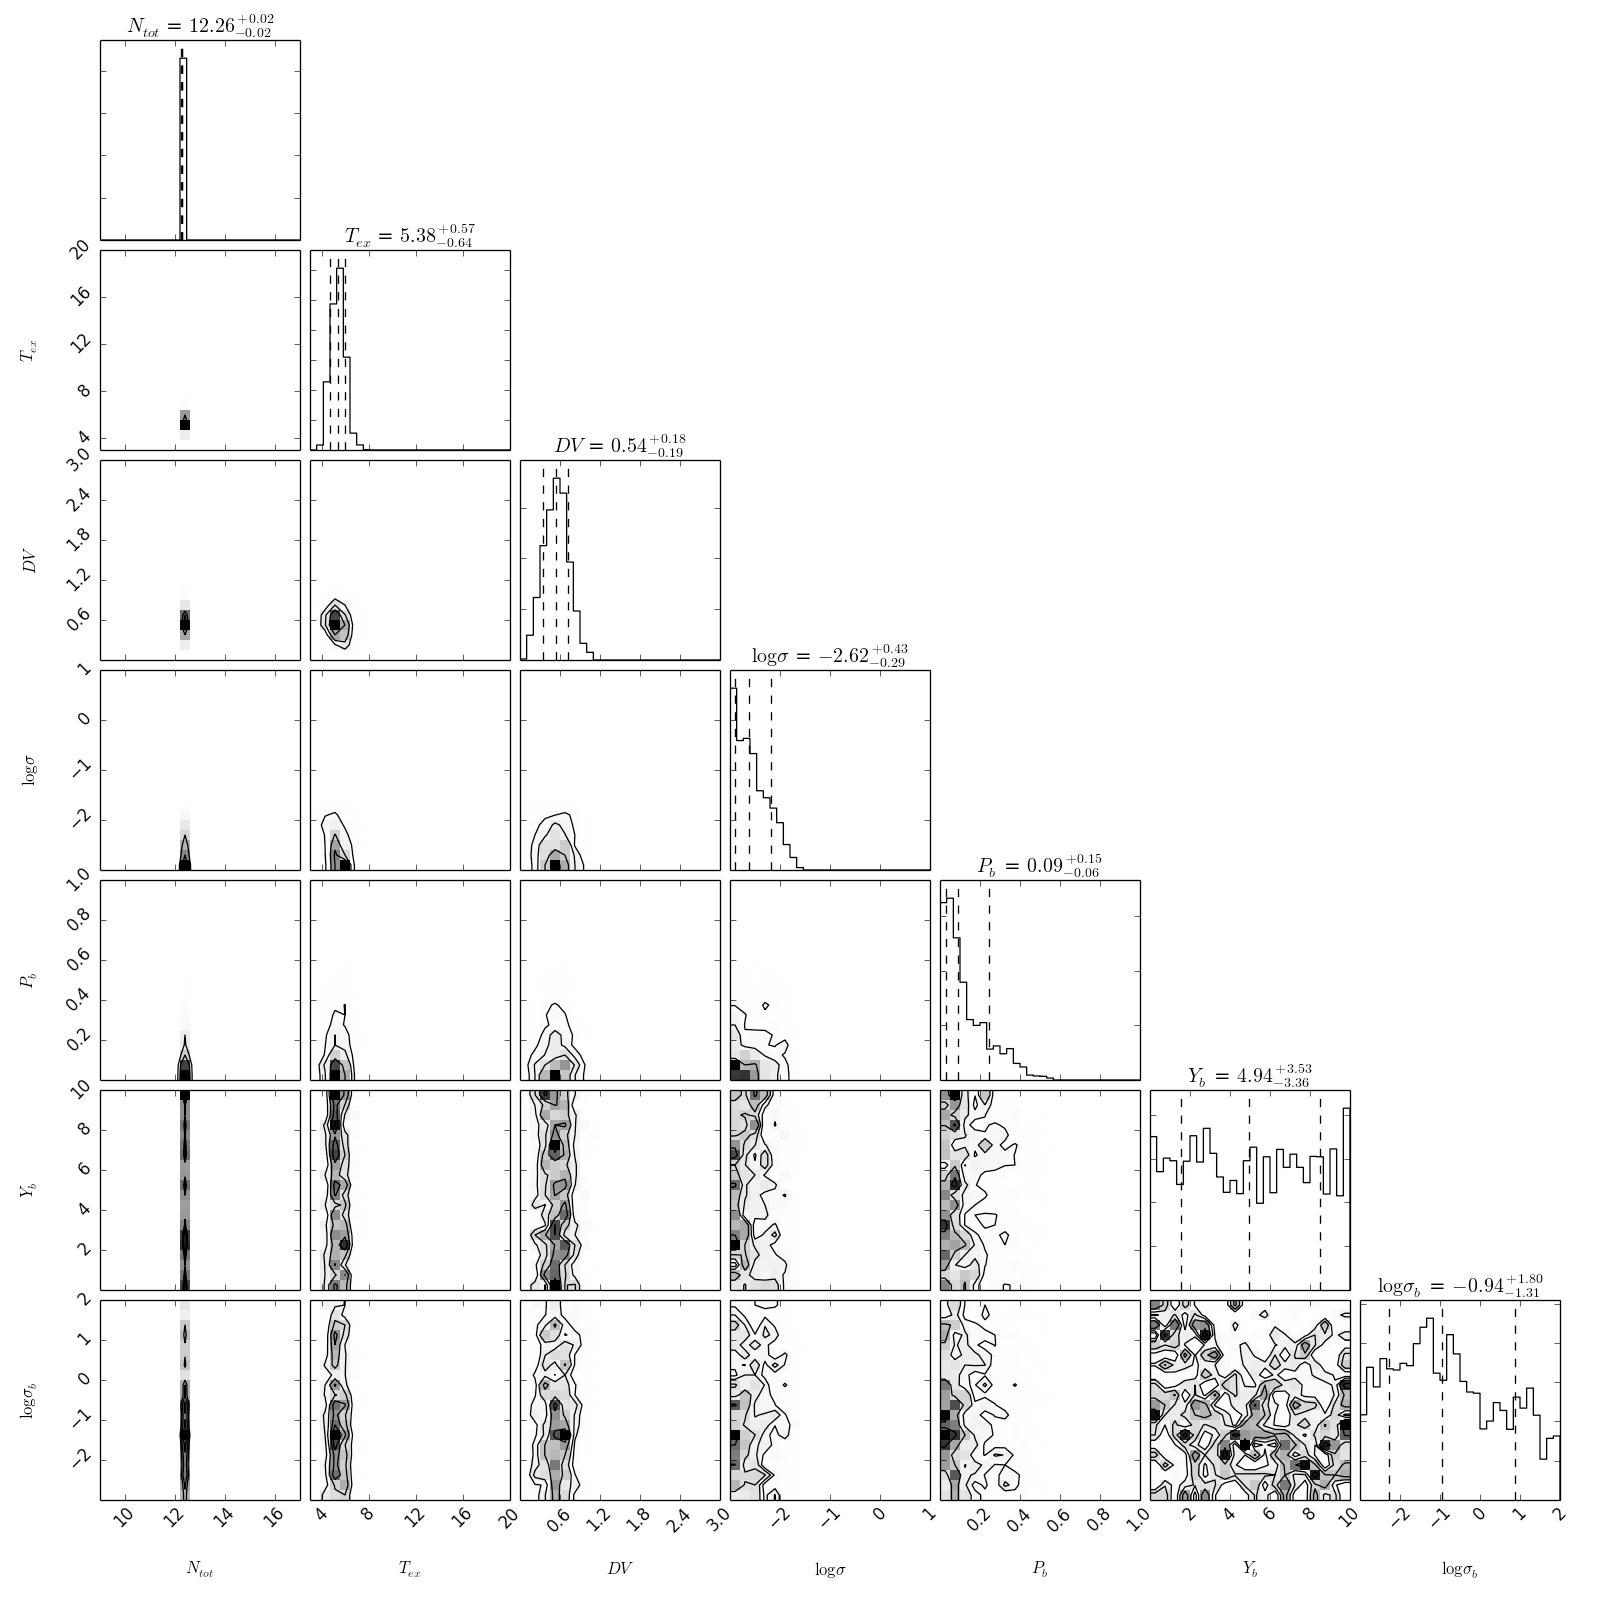}
\includegraphics[width=8cm]{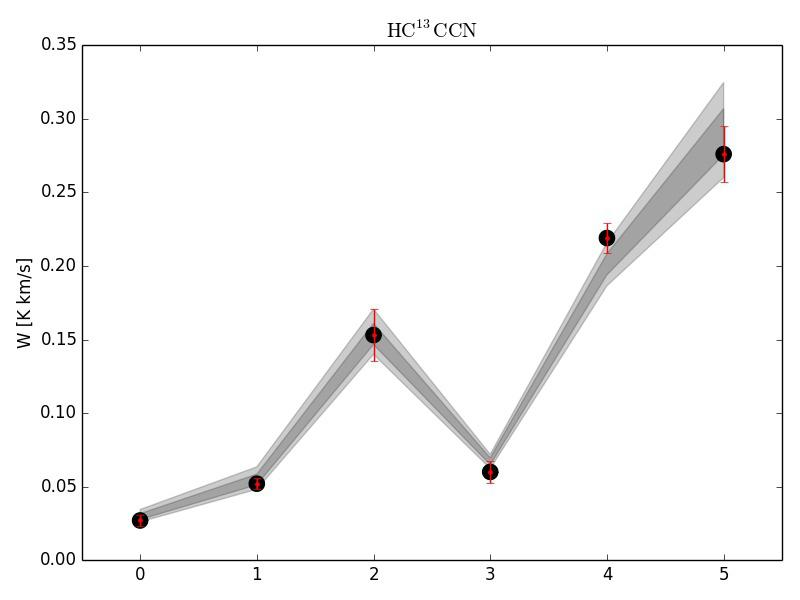}
\includegraphics[width=8cm]{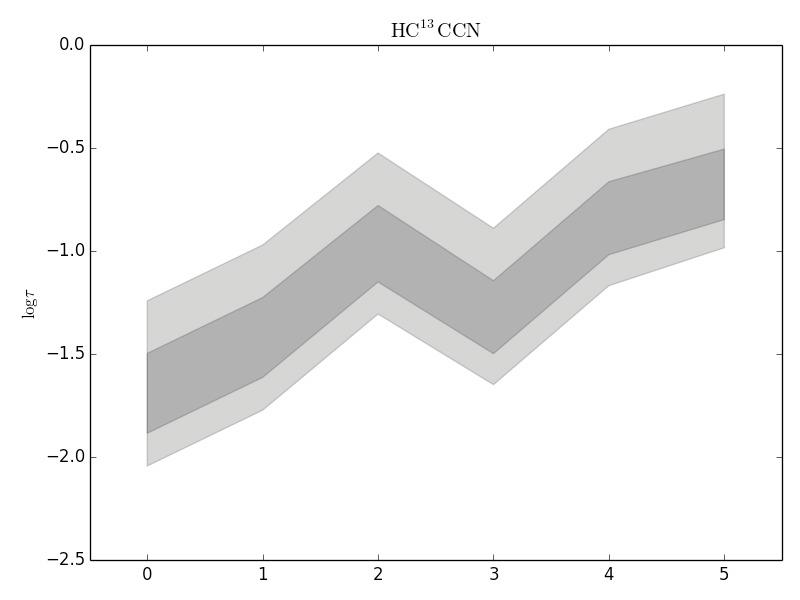}
\caption{\chem{HC^{13}CCN}}
\label{HC13CCN}
\end{figure*}
\clearpage
\begin{figure*}
\includegraphics[width=16cm]{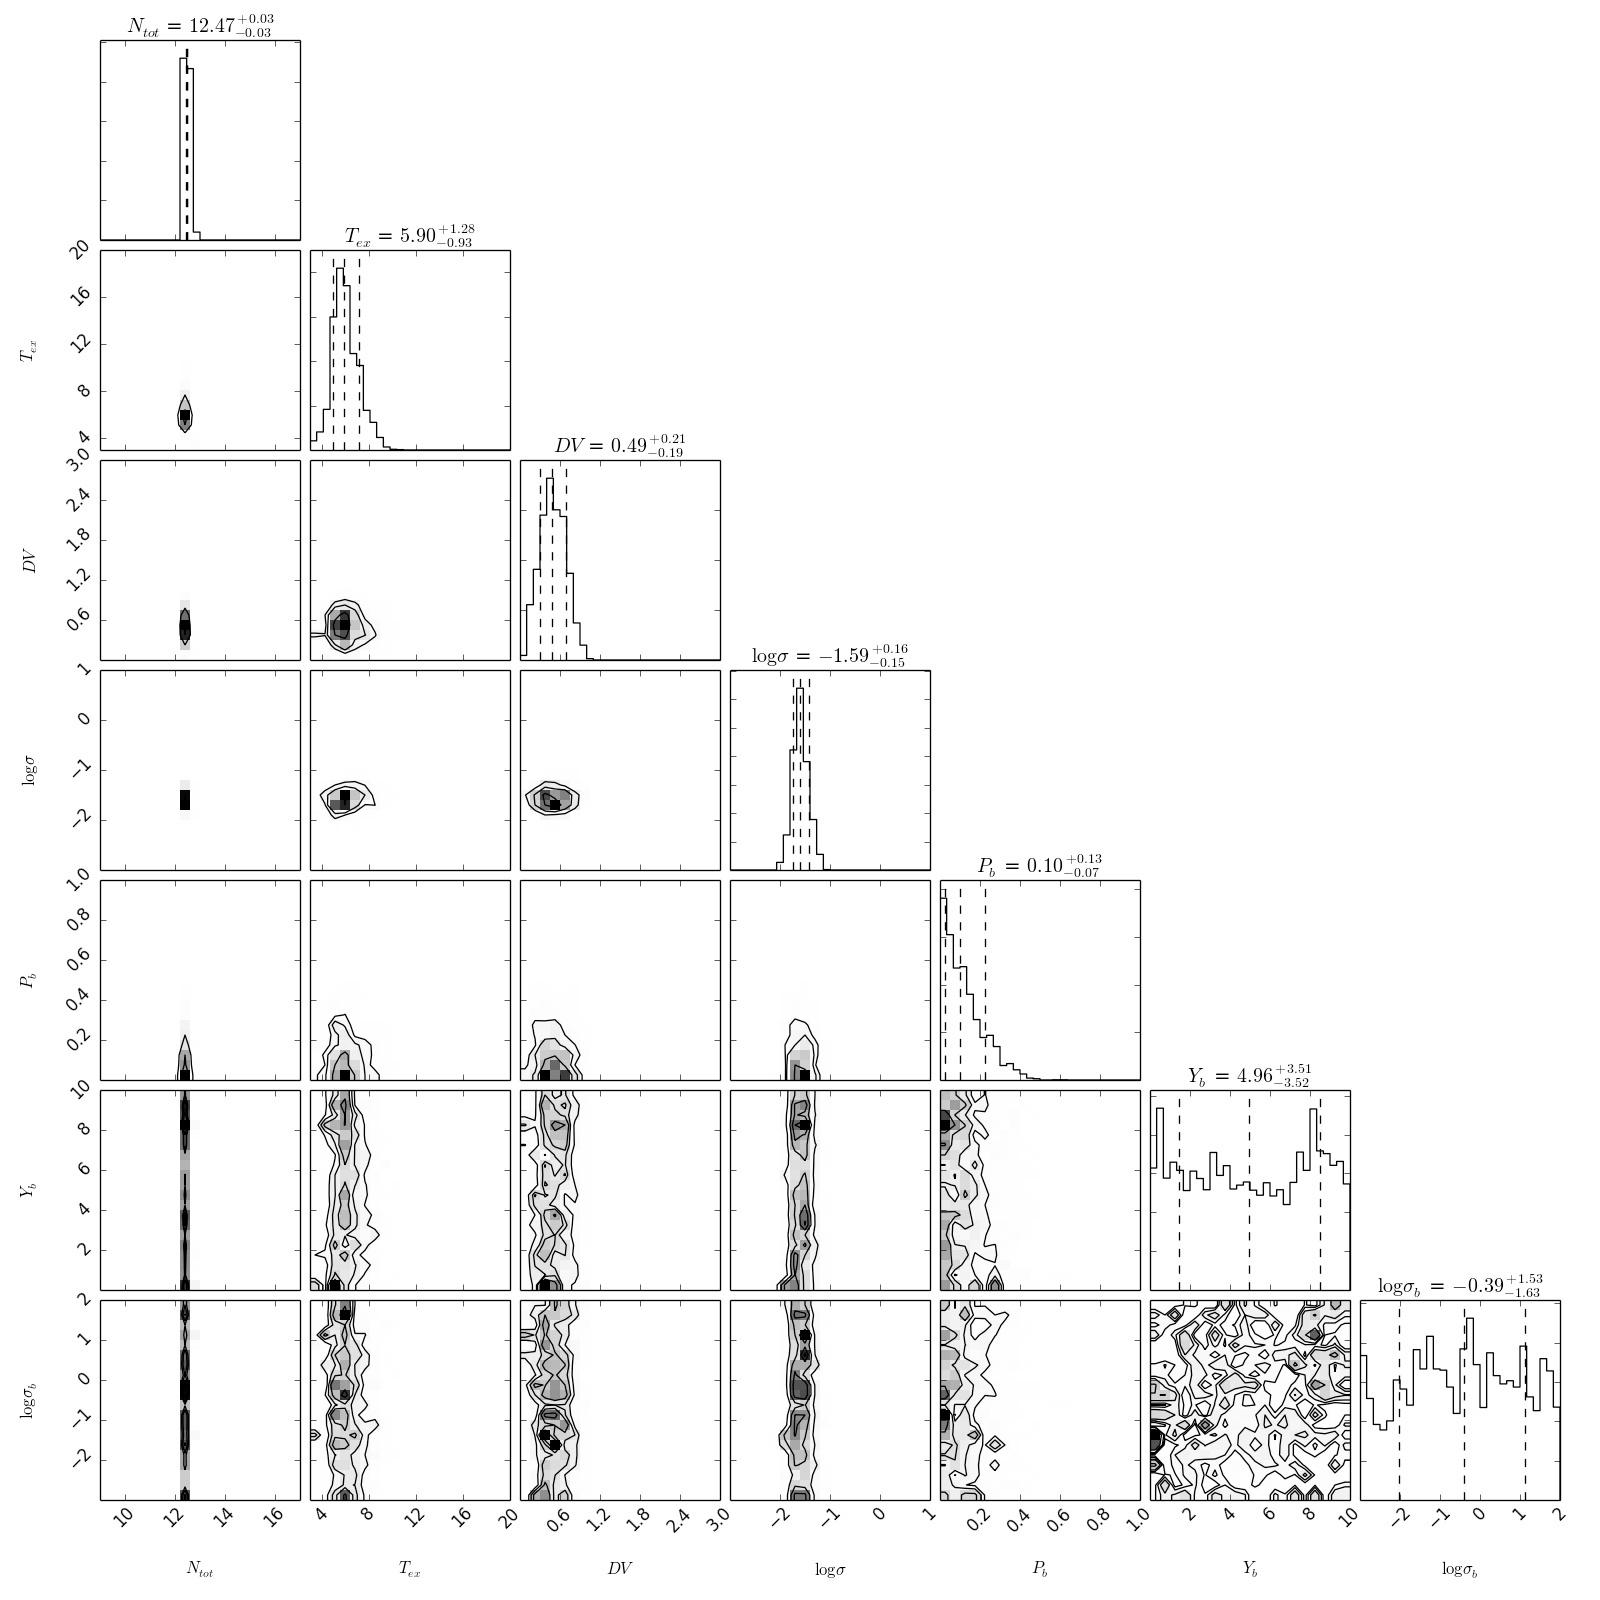}
\includegraphics[width=8cm]{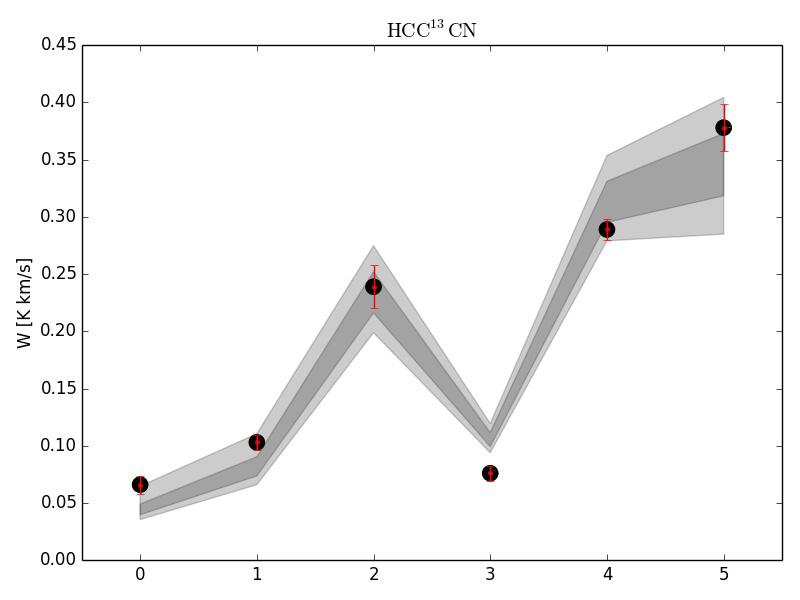}
\includegraphics[width=8cm]{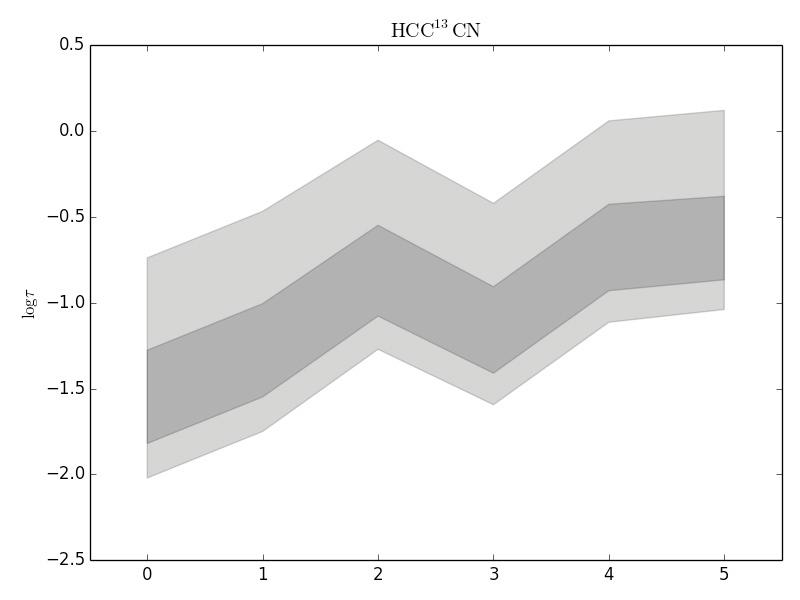}
\caption{\chem{HC_2^{13}CN}}
\label{HCC13CN}
\end{figure*}
\clearpage
\begin{figure*}
\includegraphics[width=16cm]{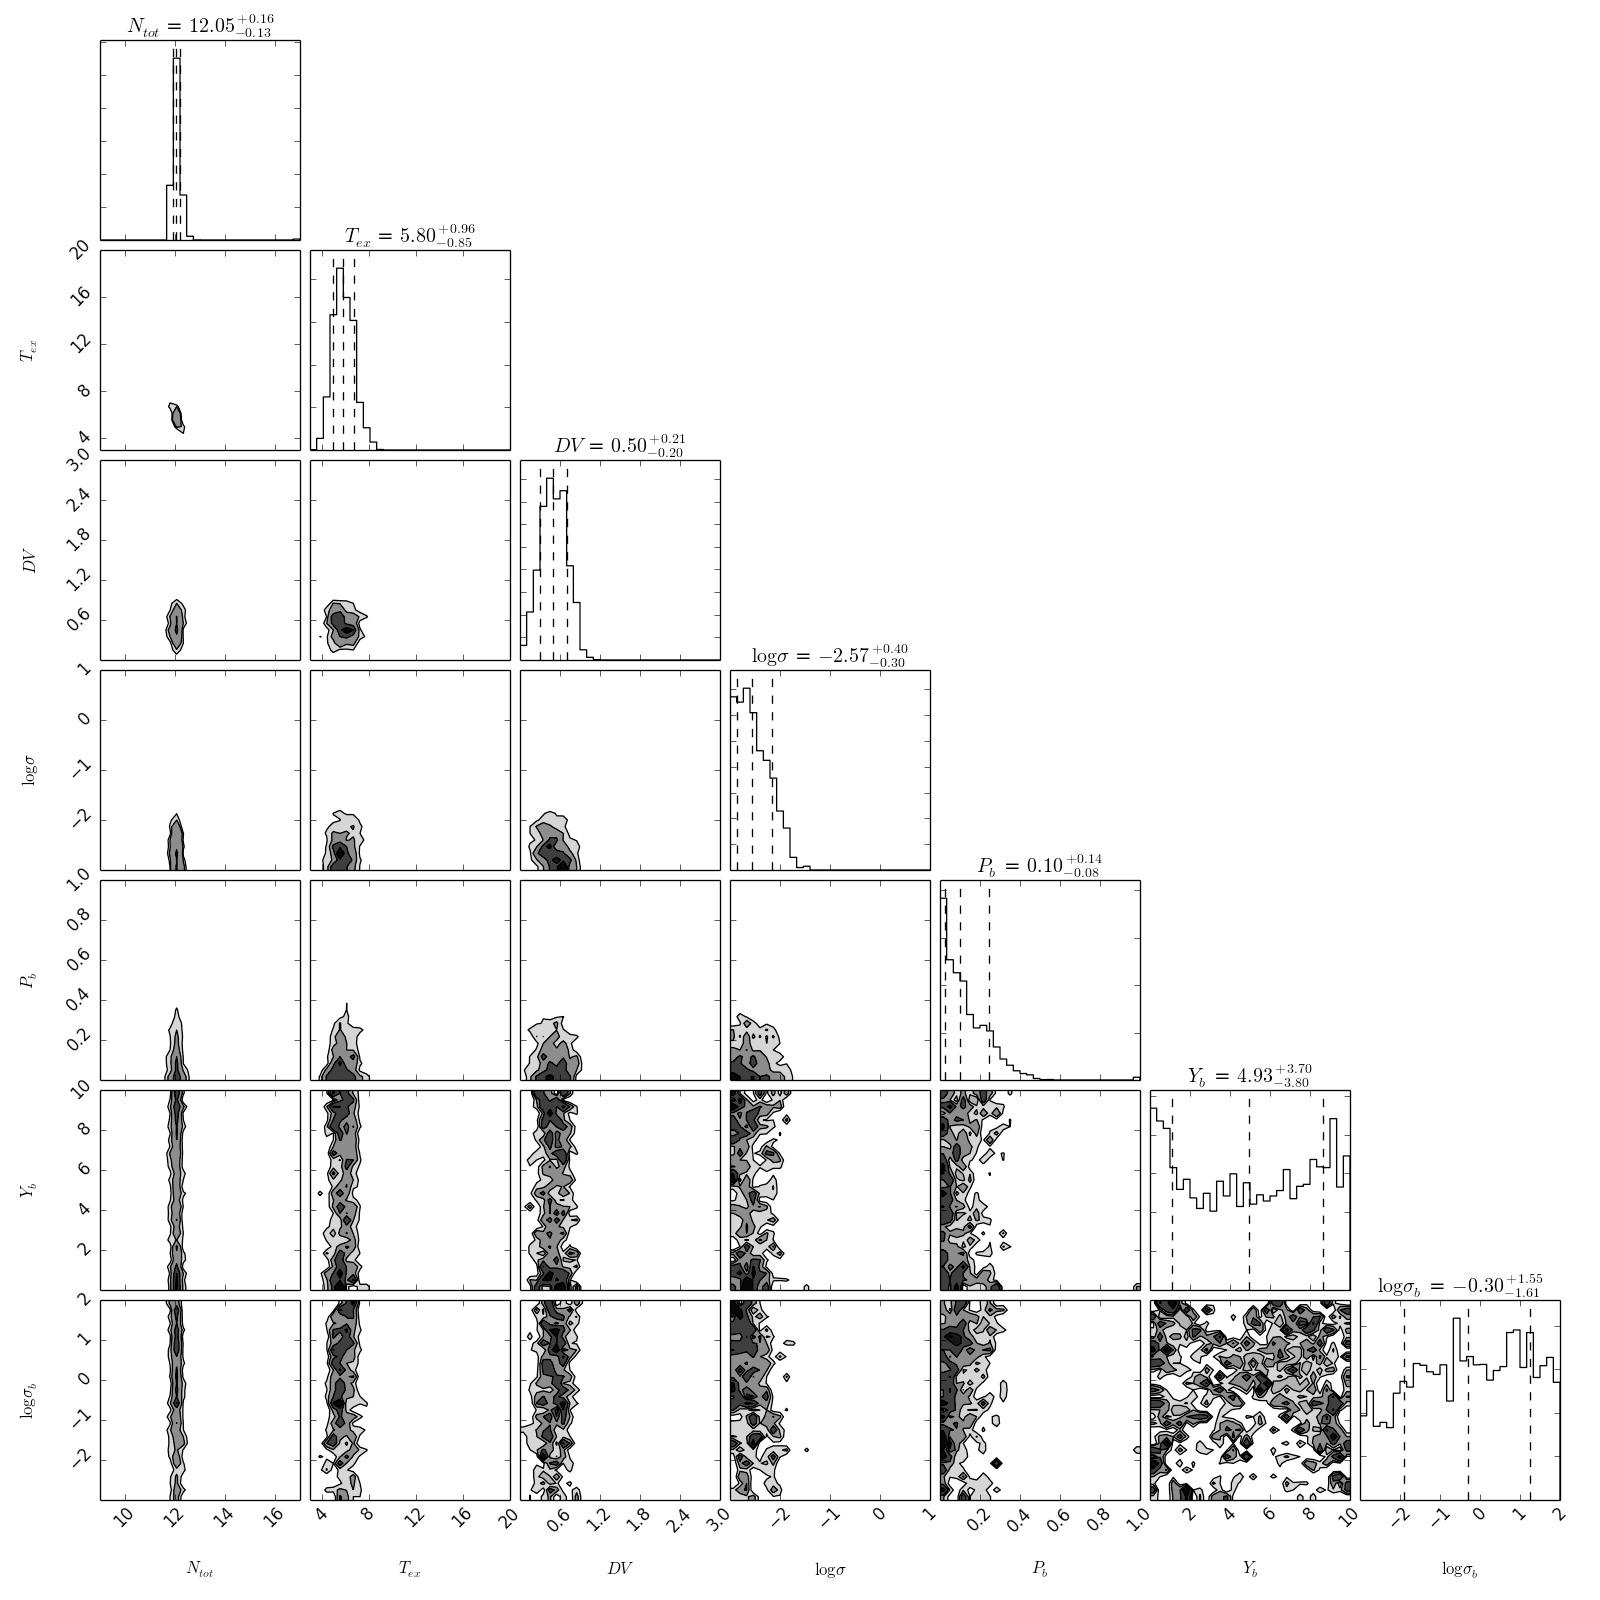}
\includegraphics[width=8cm]{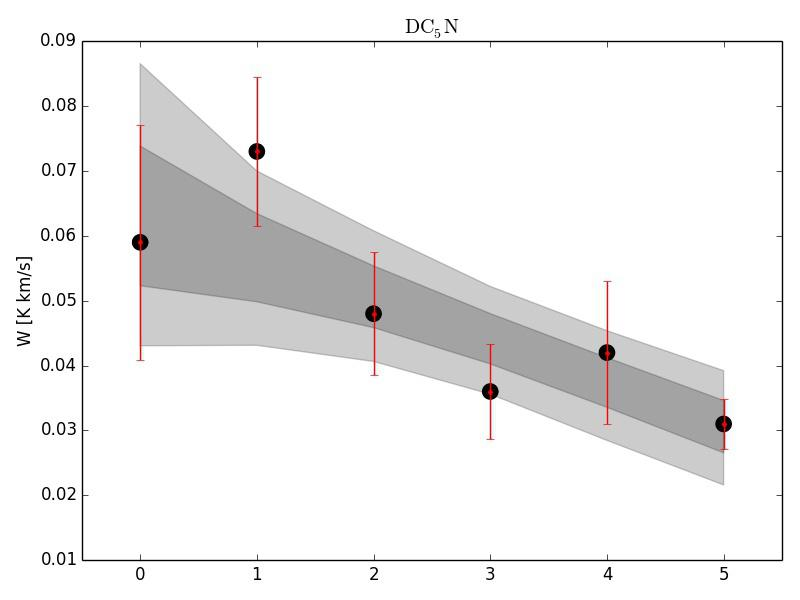}
\includegraphics[width=8cm]{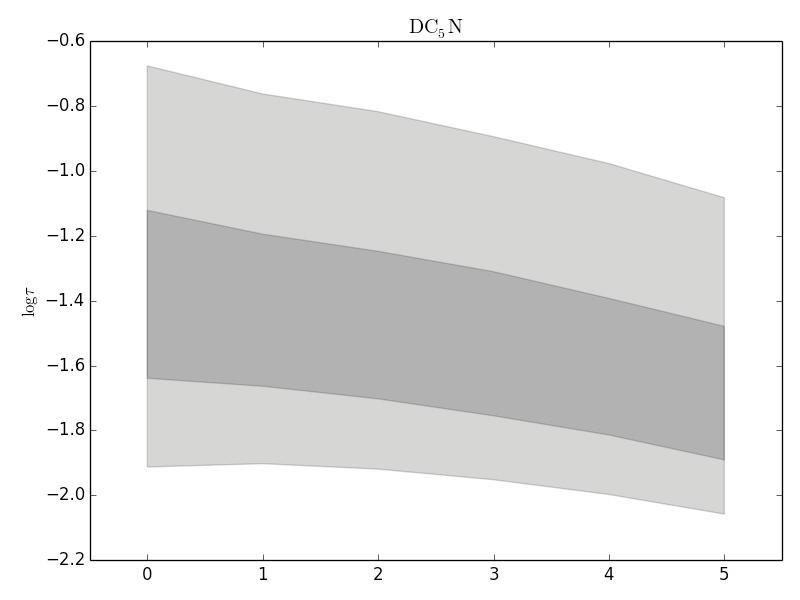}
\caption{\chem{DC_5N}}
\label{DC5N}
\end{figure*}
\clearpage
\begin{figure*}
\includegraphics[width=16cm]{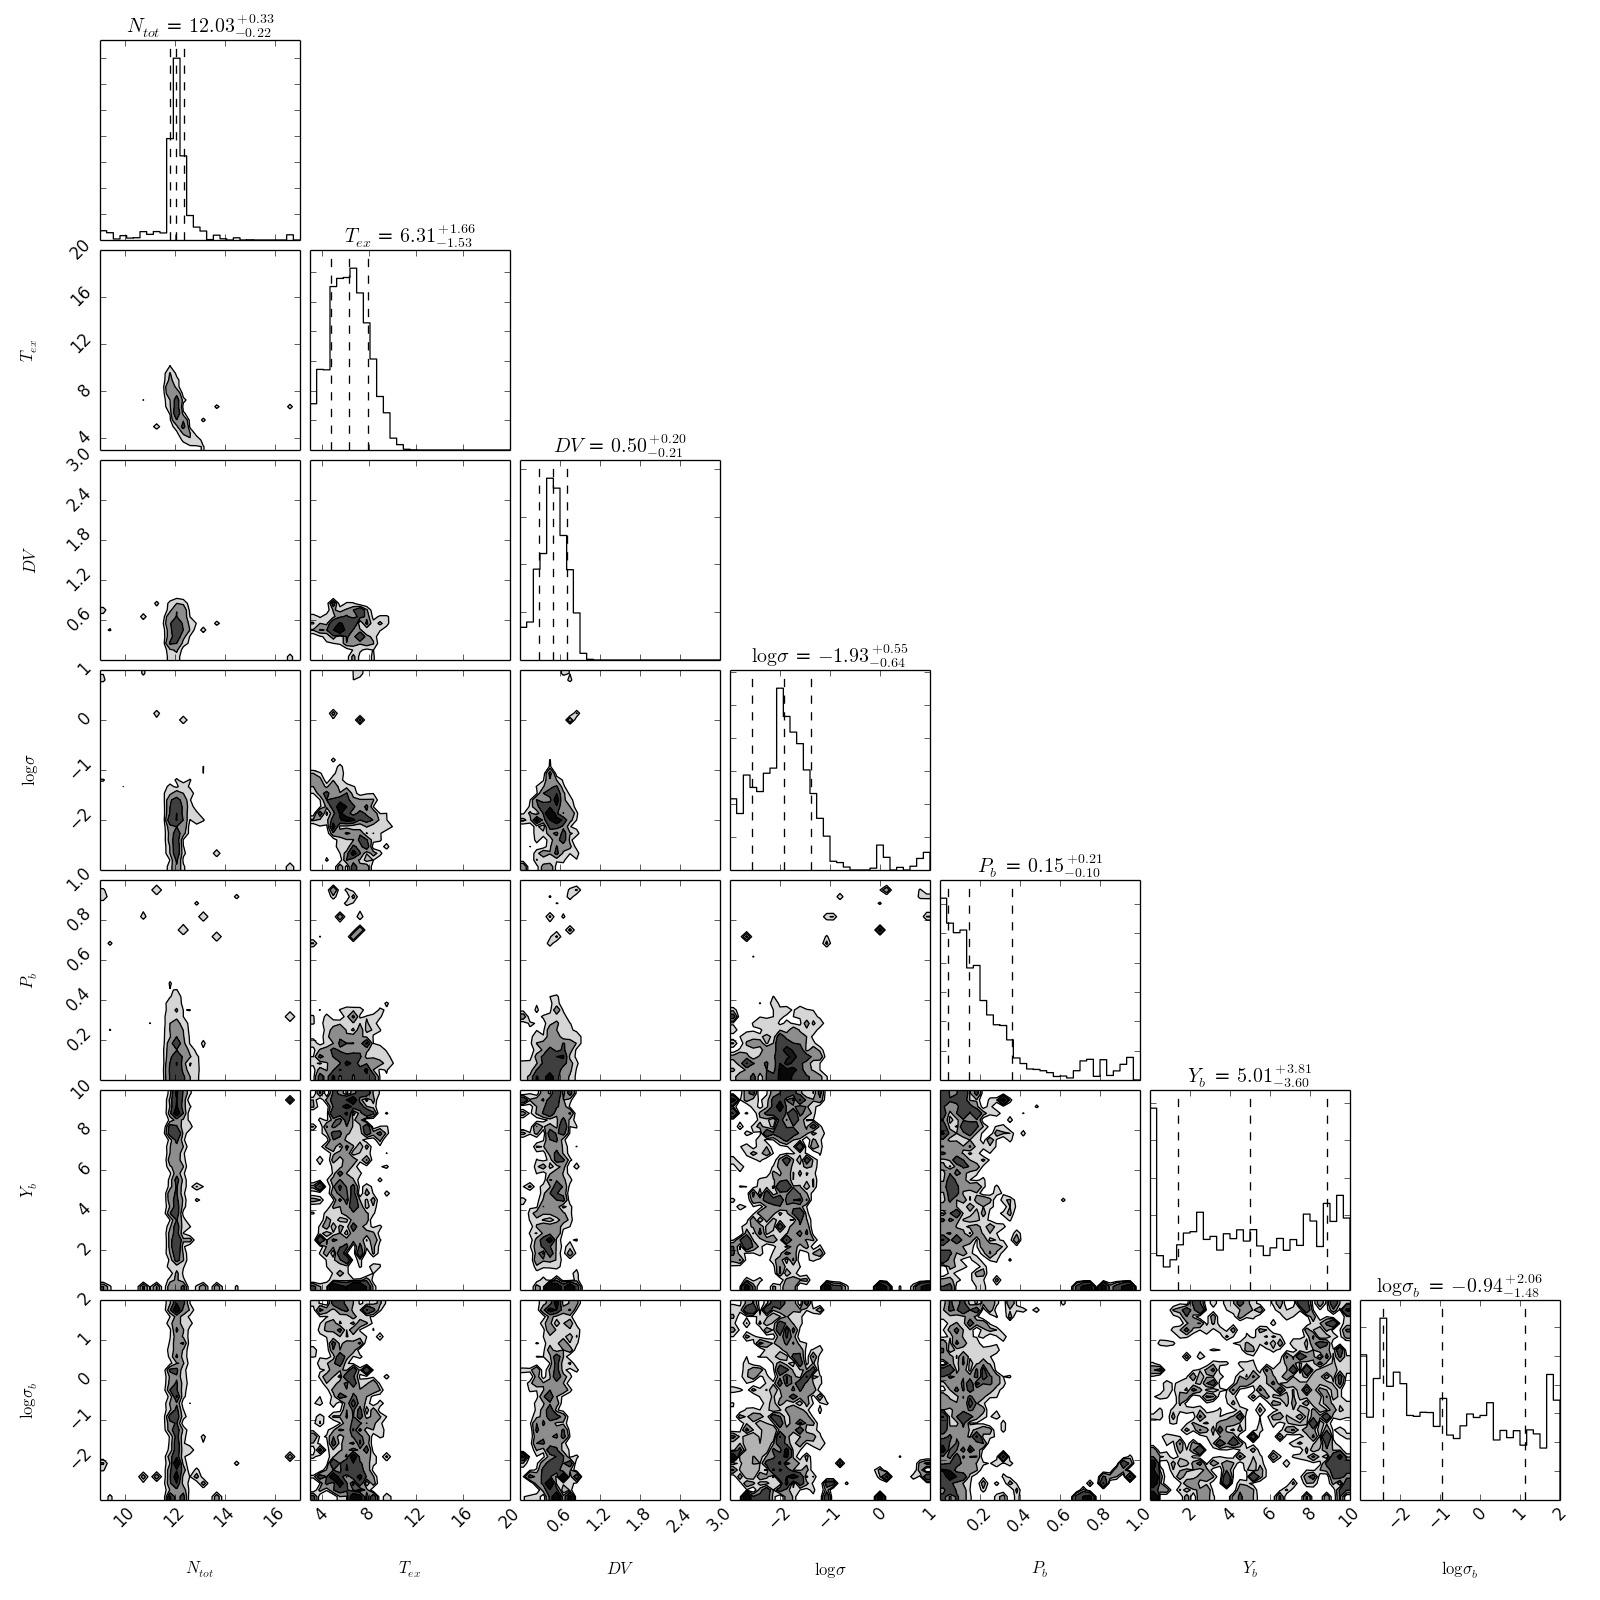}
\includegraphics[width=8cm]{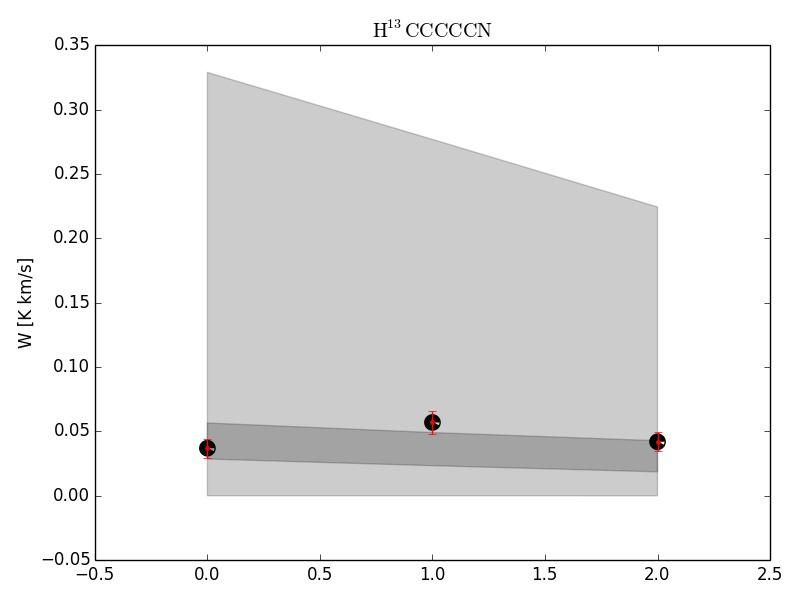}
\includegraphics[width=8cm]{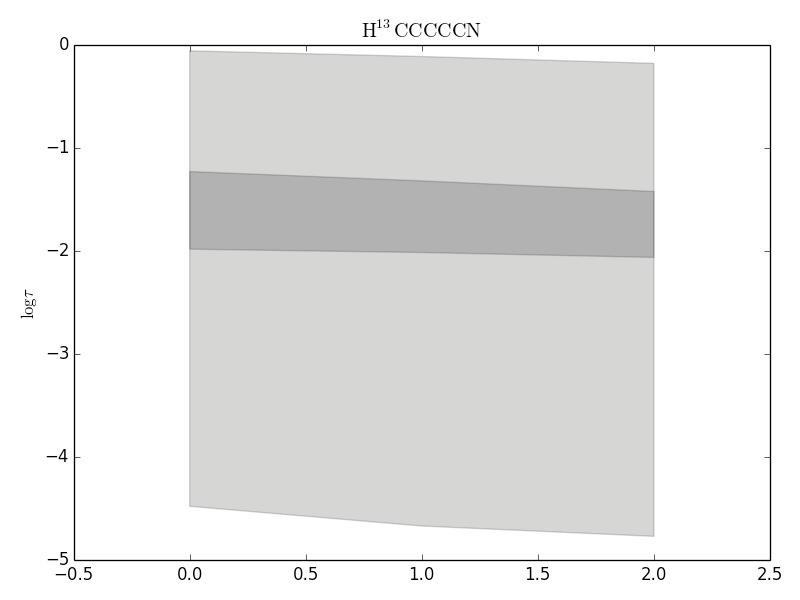}
\caption{\chem{H^{13}CC_4N}}
\label{H13CCCCCN}
\end{figure*}
\clearpage
\begin{figure*}
\includegraphics[width=16cm]{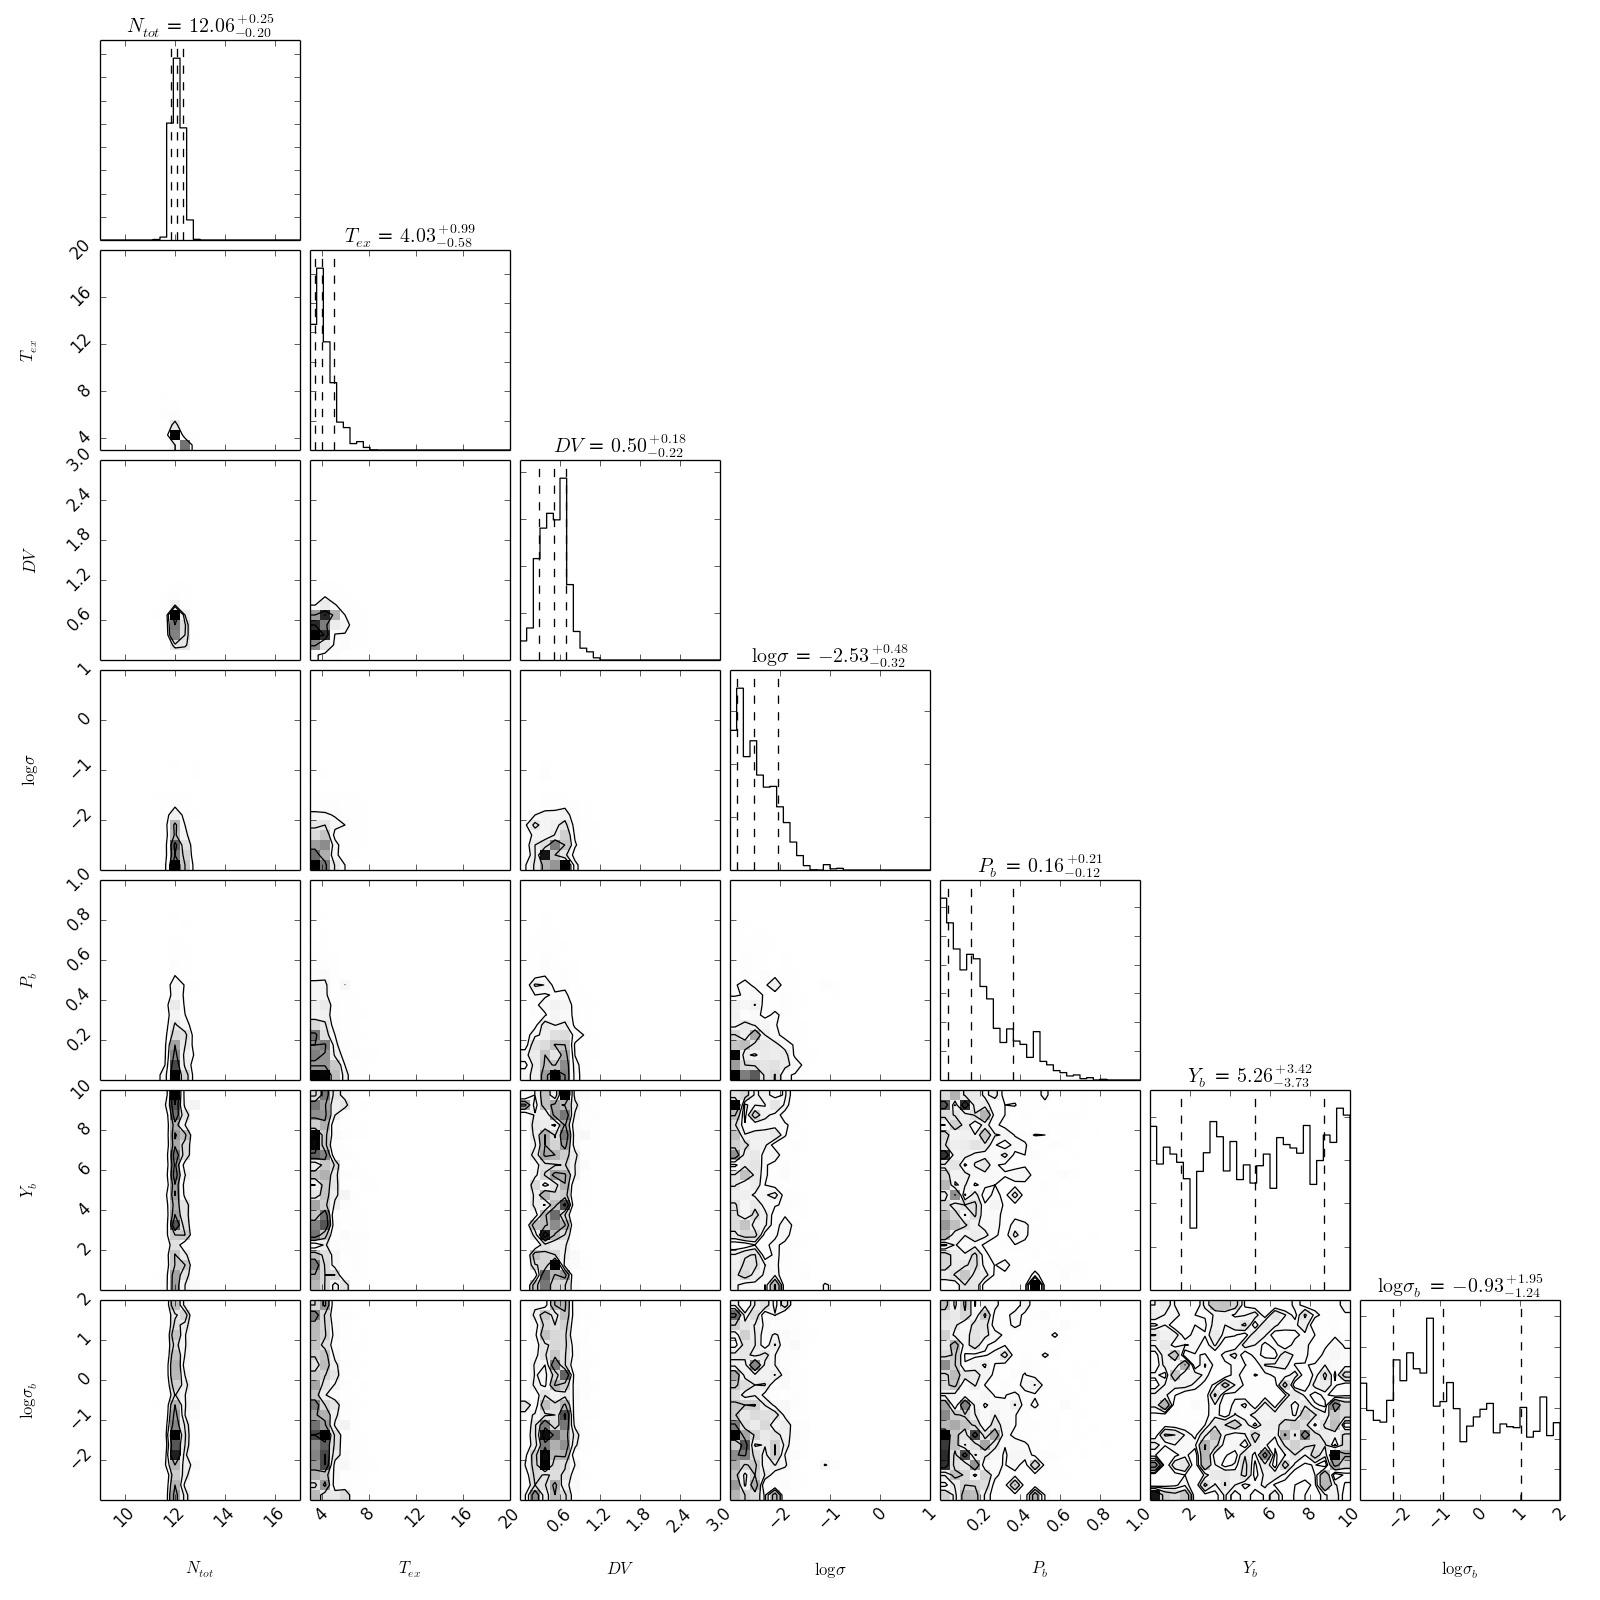}
\includegraphics[width=8cm]{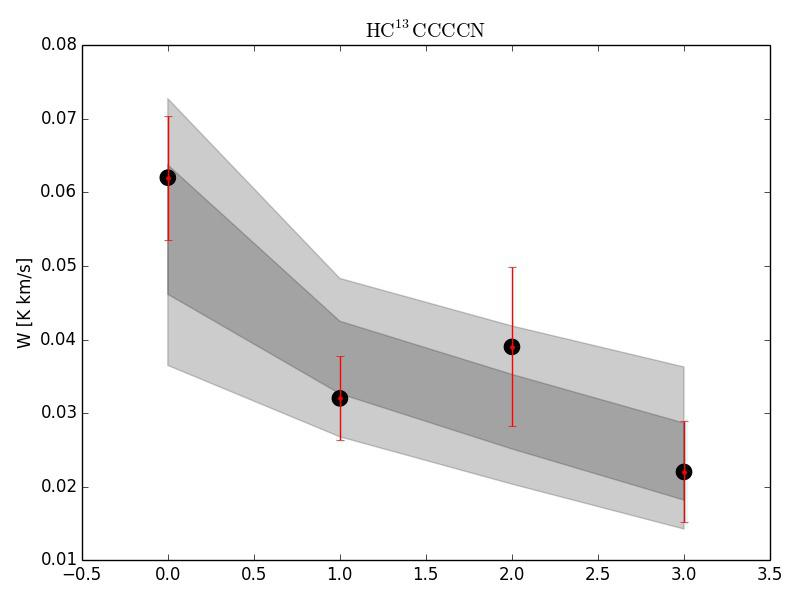}
\includegraphics[width=8cm]{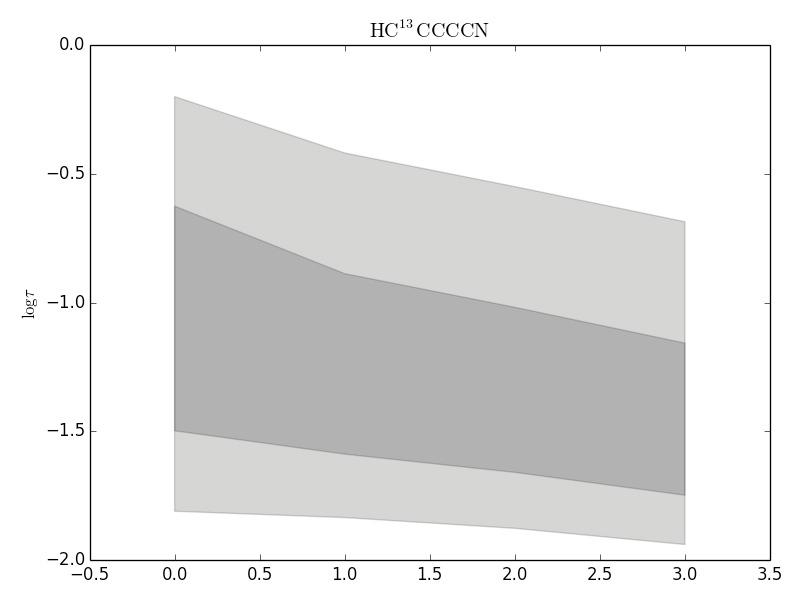}
\caption{\chem{HC^{13}CC_3N}}
\label{HC13CCCCN}
\end{figure*}
\clearpage
\begin{figure*}
\includegraphics[width=16cm]{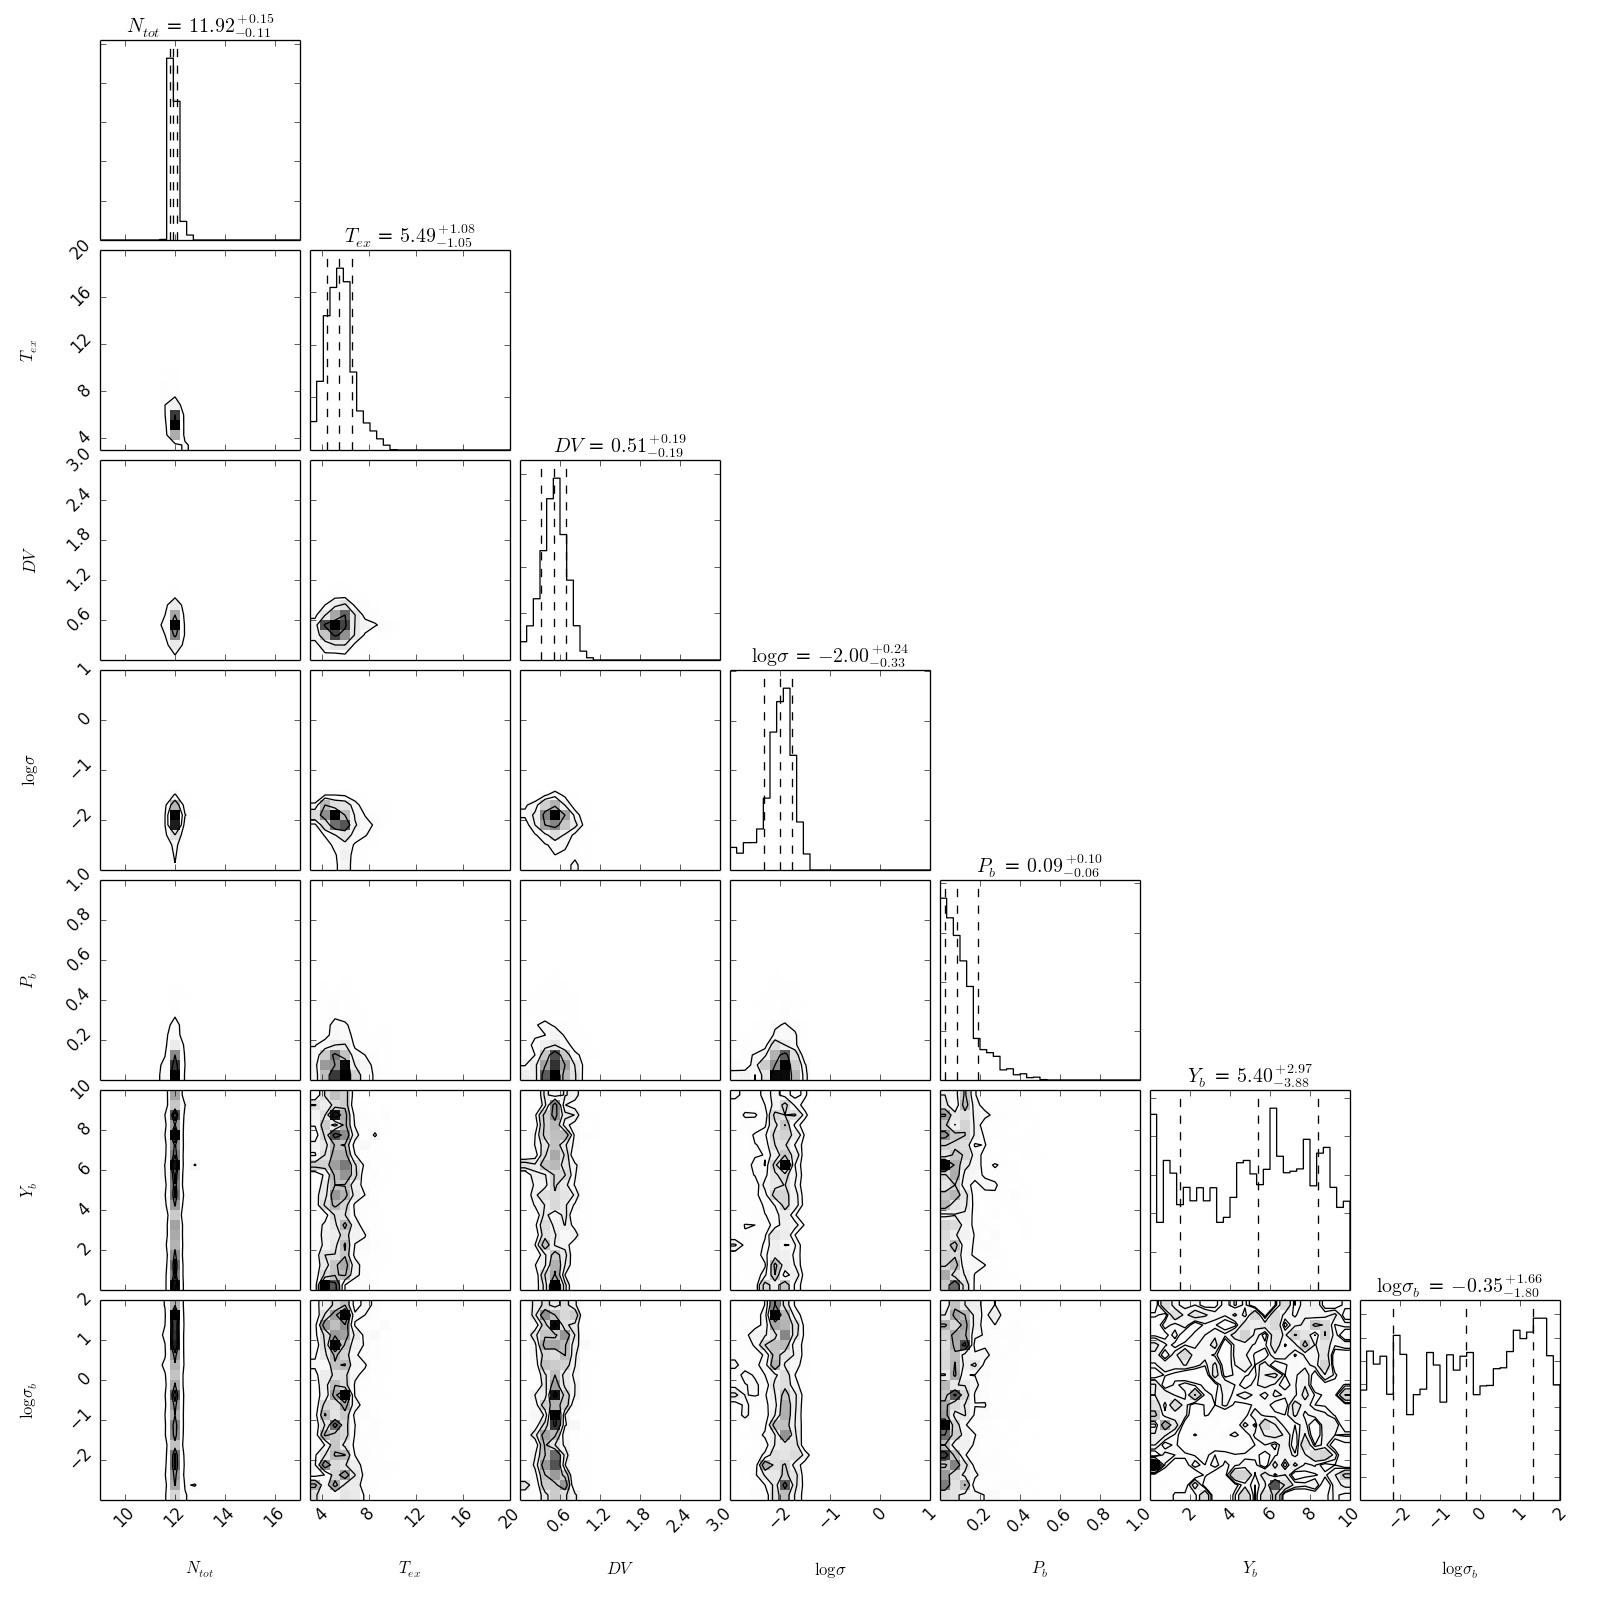}
\includegraphics[width=8cm]{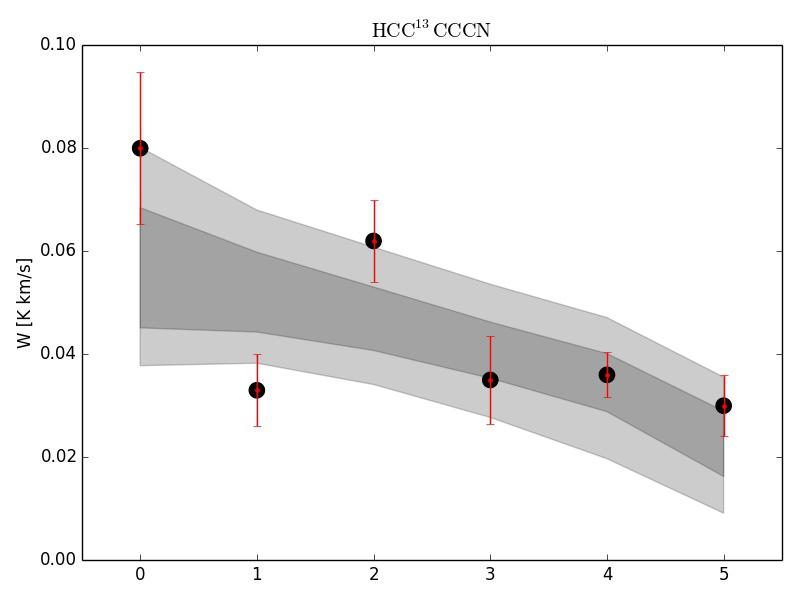}
\includegraphics[width=8cm]{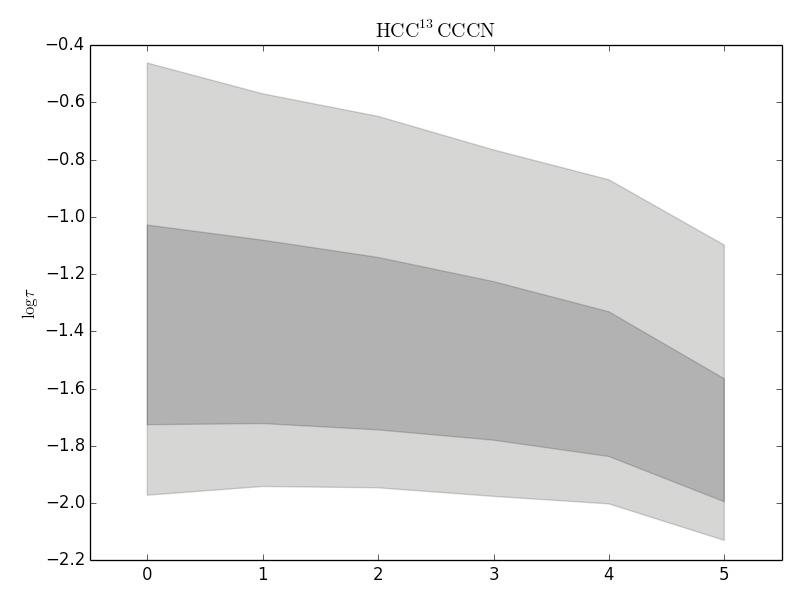}
\caption{\chem{HC_2^{13}CC_2N}}
\label{HCC13CCCN}
\end{figure*}
\clearpage
\begin{figure*}
\includegraphics[width=16cm]{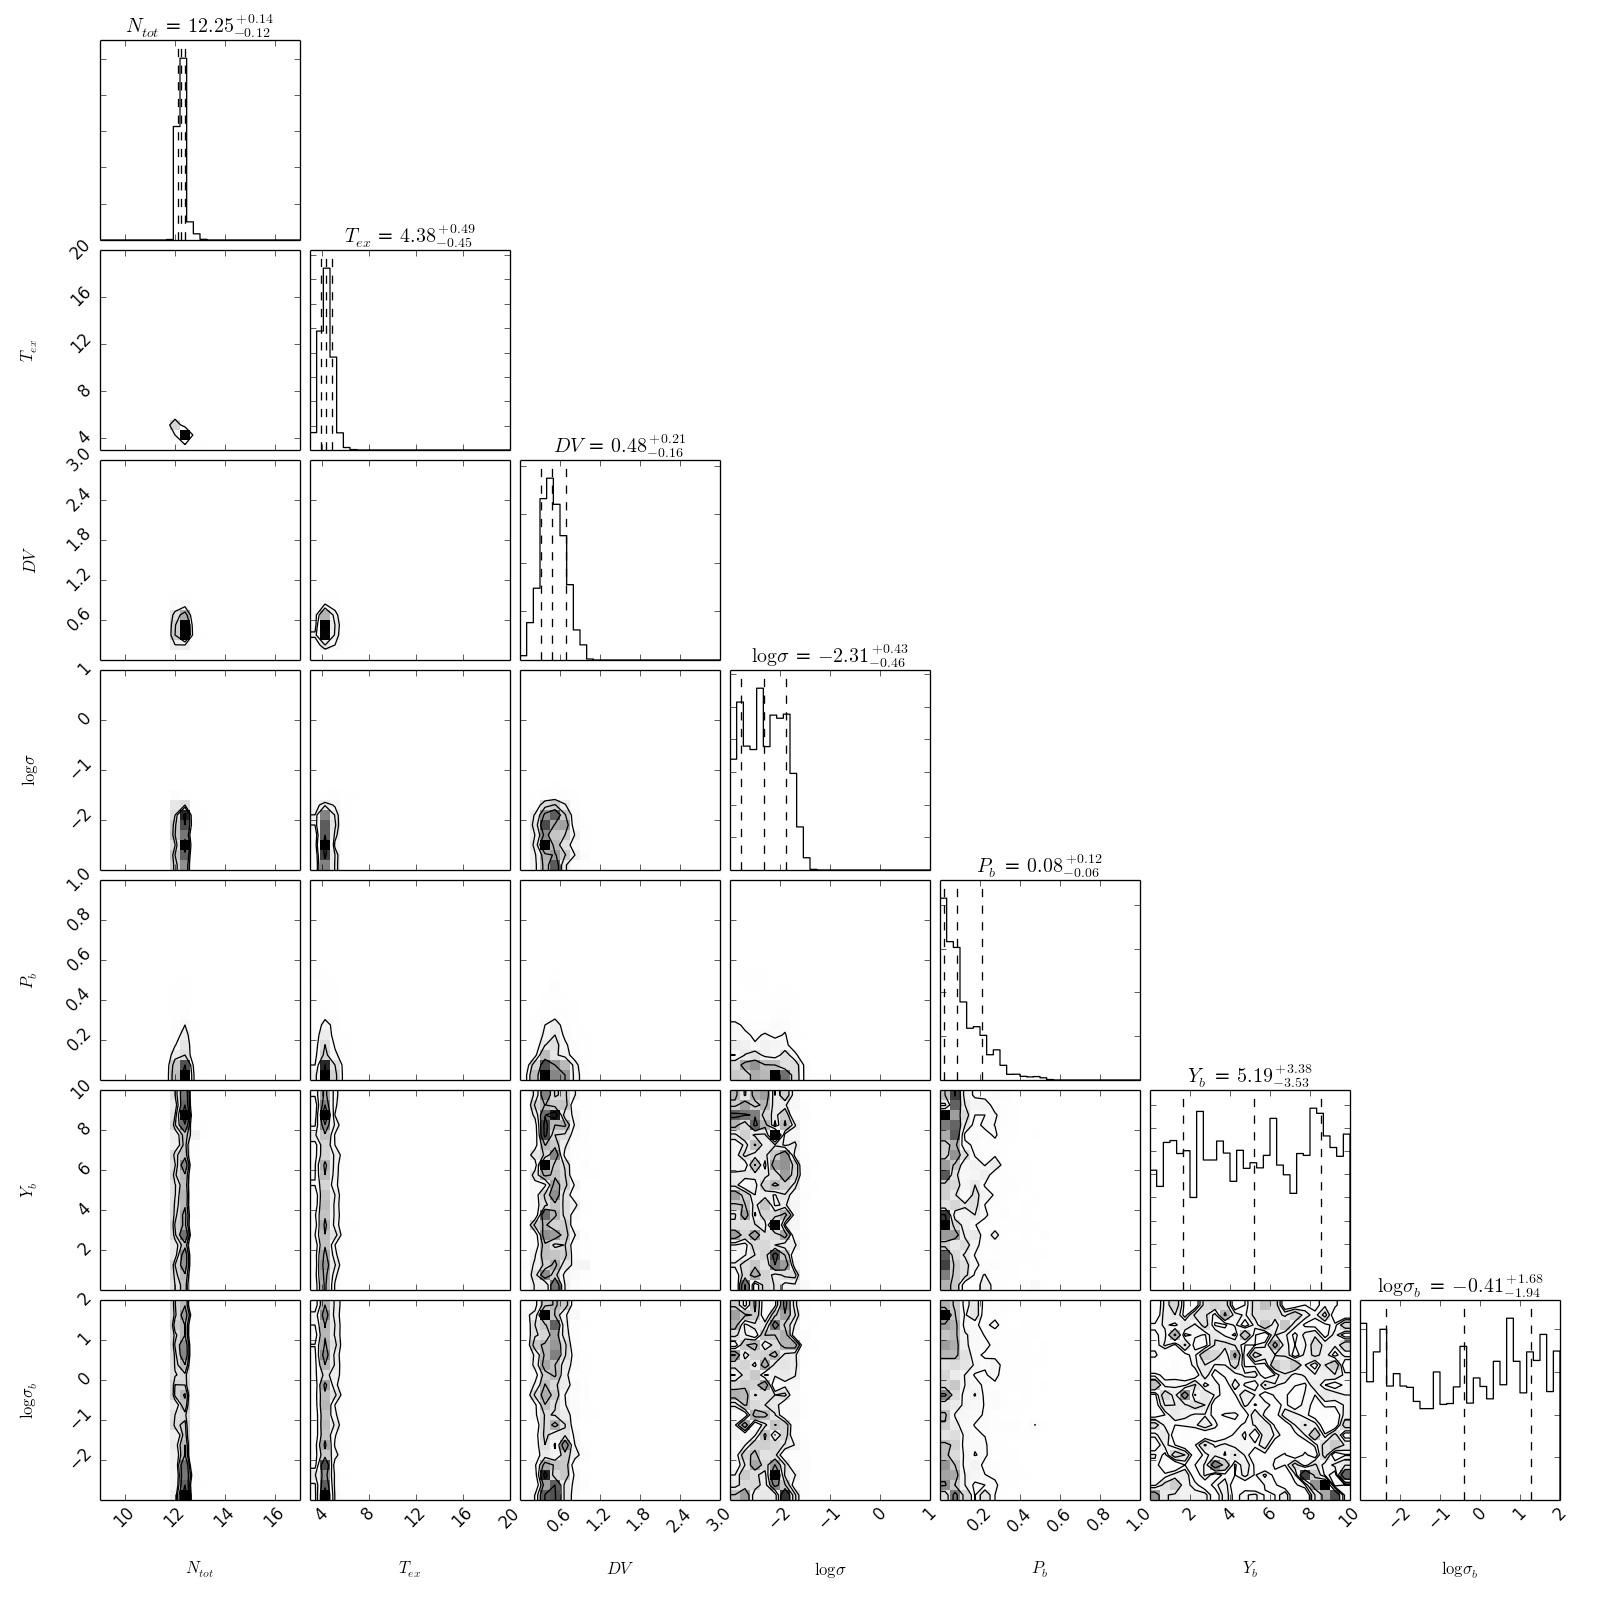}
\includegraphics[width=8cm]{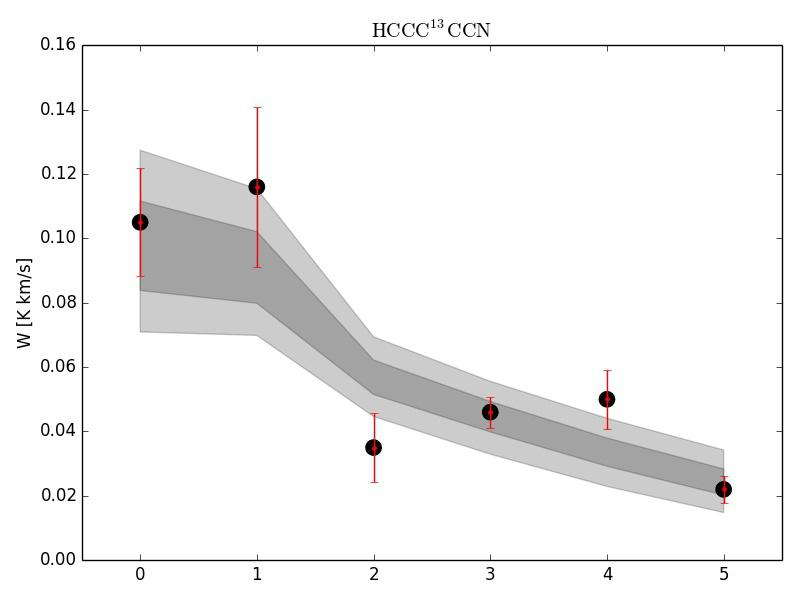}
\includegraphics[width=8cm]{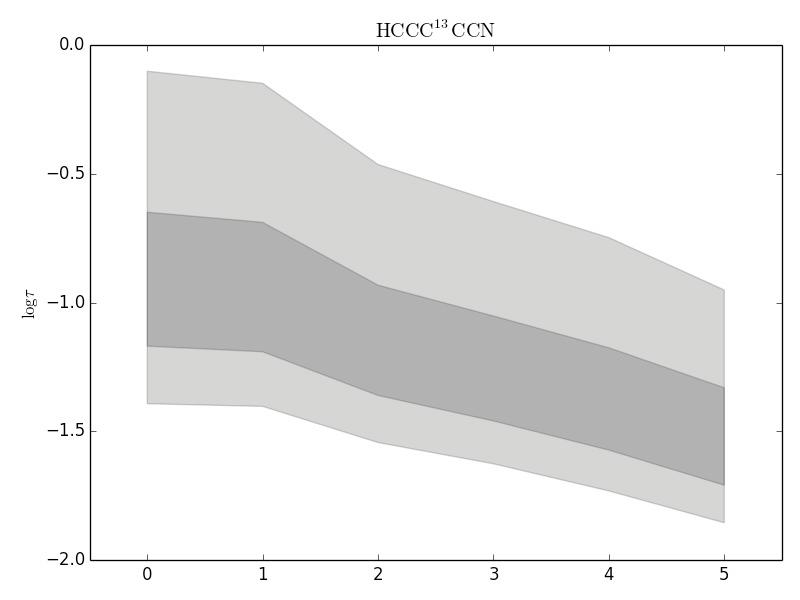}
\caption{\chem{HC_3^{13}CCN}}
\label{HCCC13CCN}
\end{figure*}
\clearpage
\begin{figure*}
\includegraphics[width=16cm]{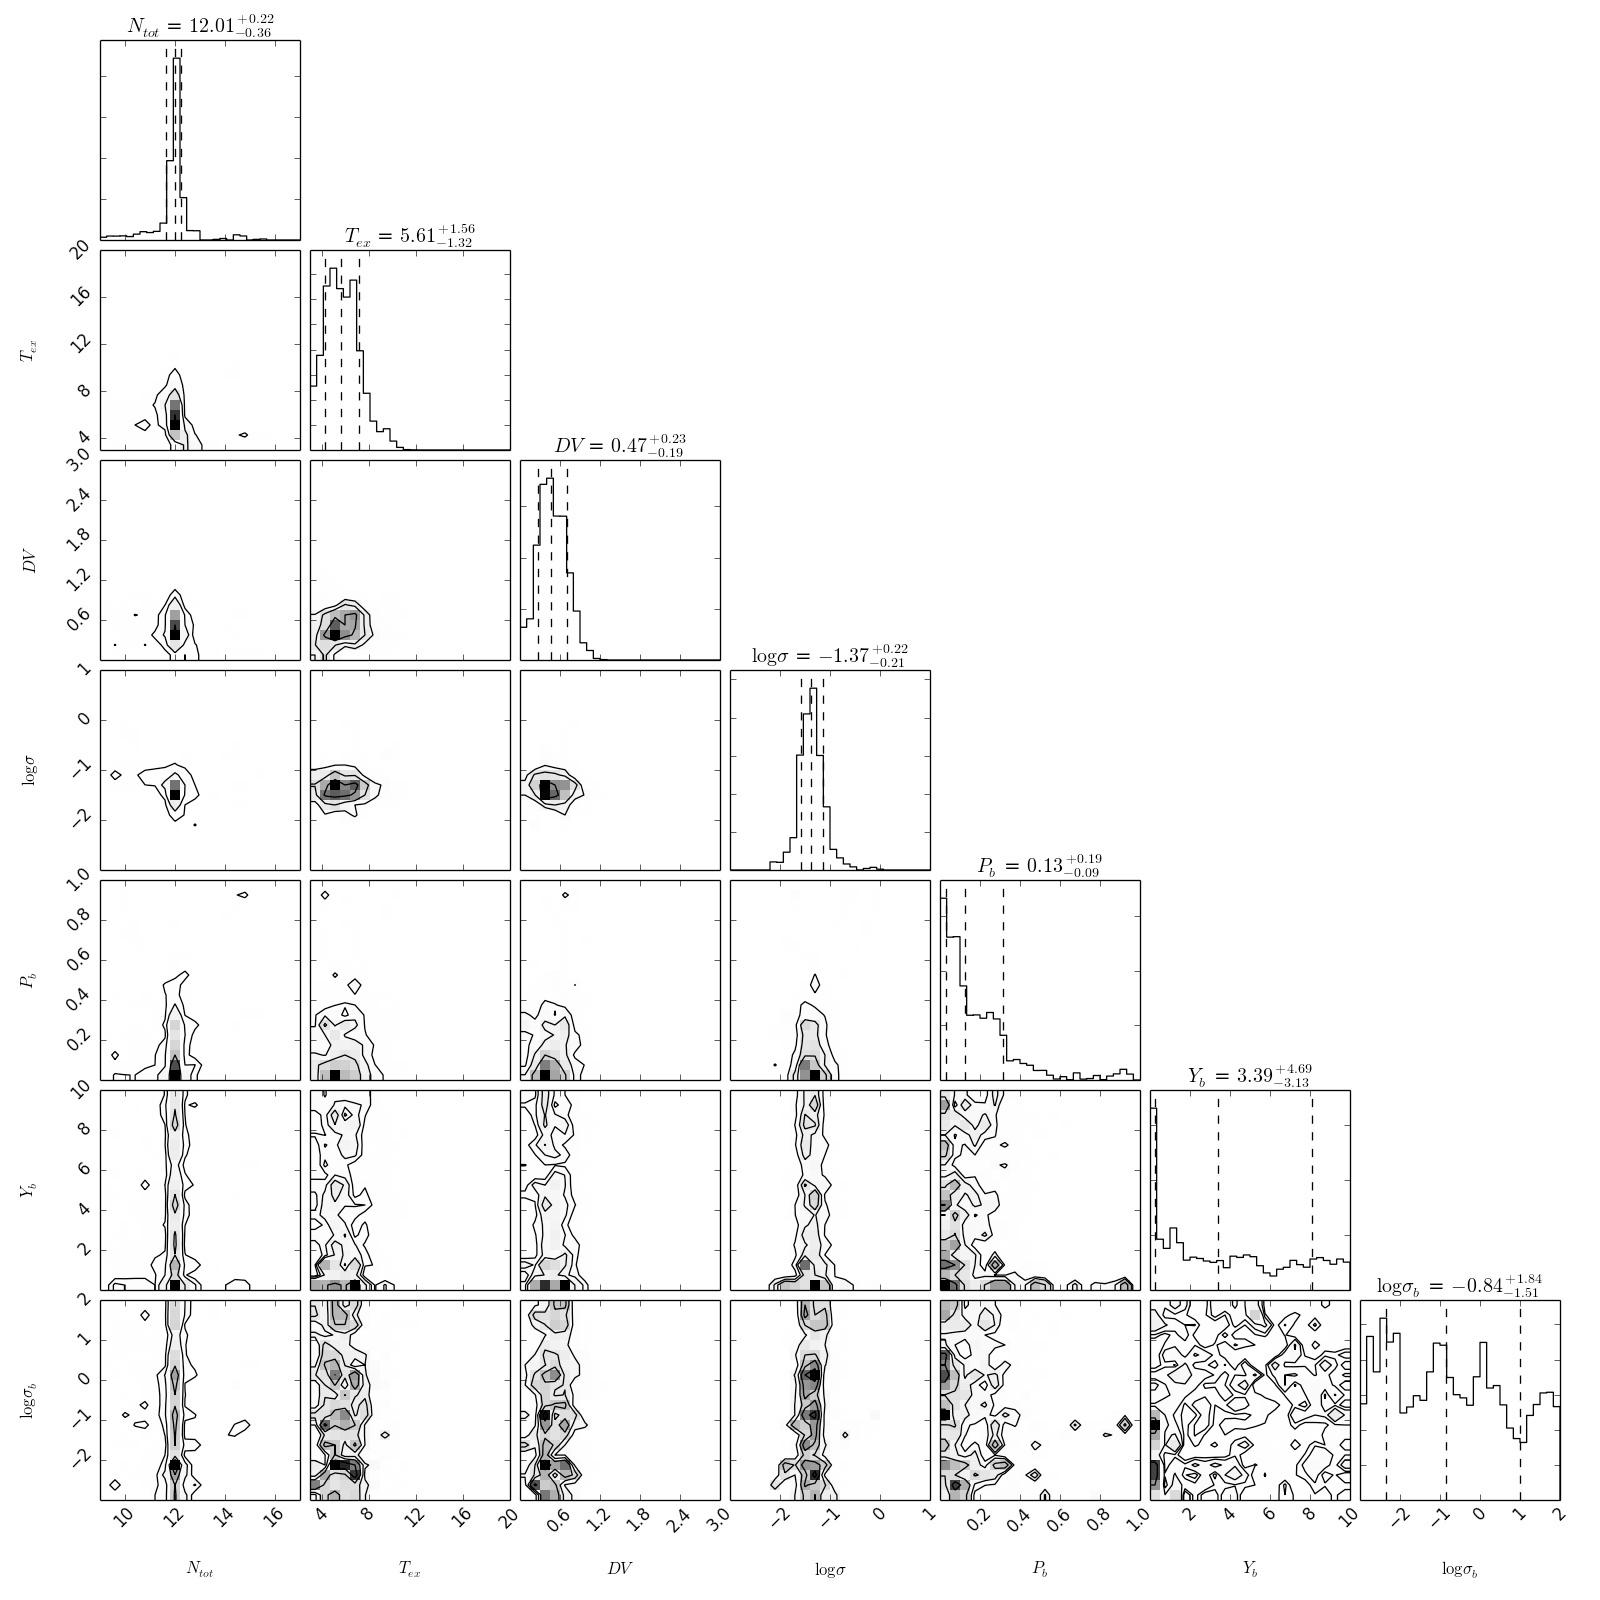}
\includegraphics[width=8cm]{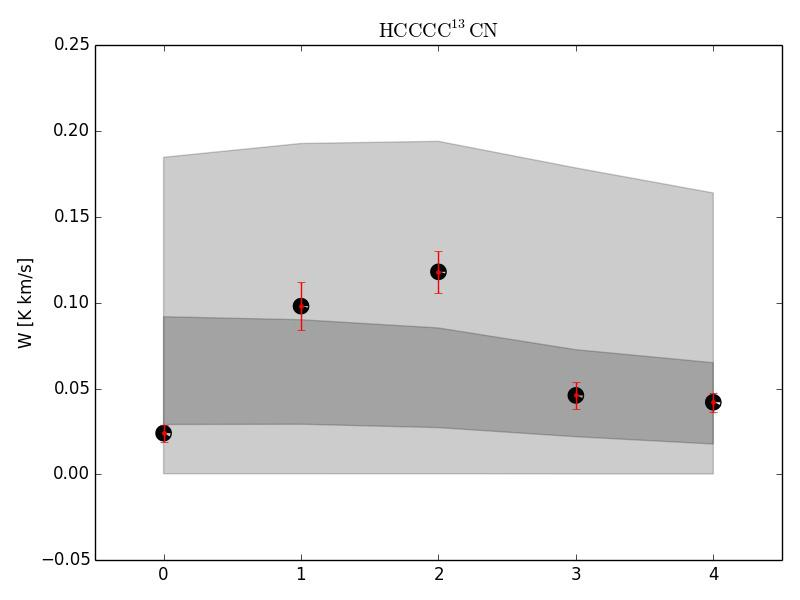}
\includegraphics[width=8cm]{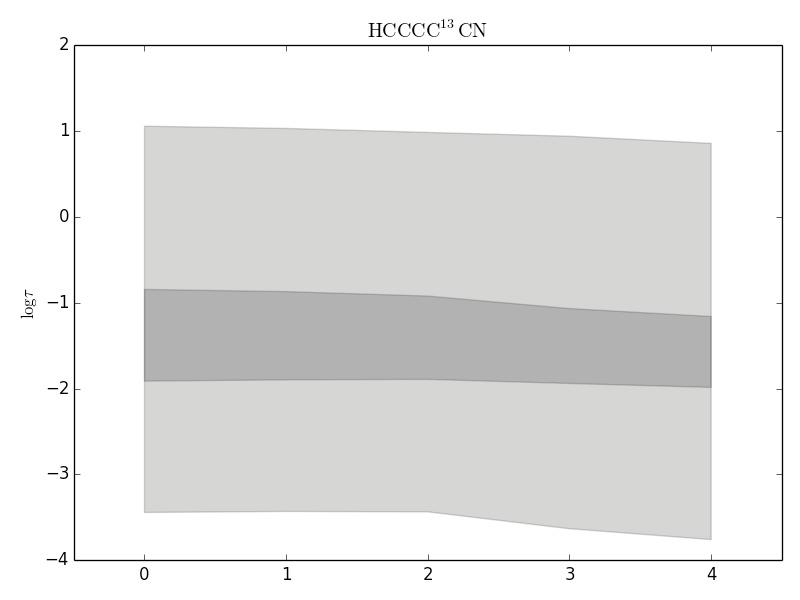}
\caption{\chem{HC_4^{13}CN}}
\label{HCCCC13CN}
\end{figure*}
\clearpage
